# Supplementary material for: Efficient, Equivariant Predictions of Distributed Charge Models
Source: arXiv:2602.07234 source file (2026-02-06)
Supplement: Supplementary file 1 [file main-si.pdf]

# Efficient, Equivariant Predictions of Distributed Charge Models

Eric D. Boittier and Markus Meuwly\*

*Department of Chemistry, University of Basel, Klingelbergstrasse 80, CH-4056 Basel, Switzerland.*

E-mail: m.meuwly@unibas.ch

## Abstract

Distributed charges model molecular electrostatic potential (ESP) anisotropy, but their transferability across chemical space remains underexplored and generation is computationally demanding. DCM-net is an equivariant graph neural network trained to construct minimal distributed charge models while preserving local symmetries, faster than computationally expensive global optimization approaches. For unseen molecules, two-charge-per-atom models achieved accuracy similar to fitted atomistic dipoles. Three- and four-charge-per-atom models reached accuracies comparable to atomistic multipole expansions up to quadrupole level, with largest gains near atoms with pronounced anisotropy (F, O) and in aromatic systems. Molecular dipole moments improved by 0.1 D versus fitted monopoles, though fitted atomistic dipoles remained more accurate. Transfer learning on dipeptides yielded 0.2 (kcal/mol)/ $e$  ESP improvement and two-fold MAE reduction in molecular dipole versus fitted monopoles. DCM-net offers a fast, physically meaningful approach to generating distributed charge models for applications including force field development and QM/MM calculations.

September 10, 2025

# 1 Introduction

The electrostatic potential (ESP) of a molecule can be used to explain many phenomena such as structure, bonding, stability, and reactivity, among others.<sup>1-5</sup> The specific orientation of intermolecular interactions is largely guided by electrostatics; however, the ESP is an anisotropic charge distribution, due to high-symmetry features of the wavefunction— often referred to as lone pairs and sigma-holes, for example.<sup>6-9</sup> By reducing the representation of the local electrostatic environment to atomic multipoles or point charges (PCs), the true anisotropic electrostatic potential of the molecule is neglected.<sup>10</sup> A successful approach to modeling the molecular electrostatic potential has been to use atom-centered multipoles (MTPs) to a given order. Often, this expansion is truncated at the atomic quadrupole moment for all atoms except hydrogens for which a PC representation is usually sufficient.<sup>10-13</sup> Including higher order atomic multipoles has been successful in crystal structure prediction<sup>14</sup> and modeling interaction energies using force fields.<sup>15-17</sup> These atomic multipole expansions can be obtained from the electron density of the wavefunction, using techniques such as the Minimal Basis Iterative Stockholder (MBIS) procedure.<sup>18</sup> Interoperable quantum-chemistry workflows and drivers such as QCDB/QCEngine facilitate automated, reproducible ESP and property evaluations across engines.<sup>19</sup>

The quantum theory of atoms in molecules (QTAIM) suggests features in the molecular density, such as bond critical points, which are well described using off-center multipoles, which has led to the development of distributed multipoles.<sup>20</sup> Likewise, PC-based energy functions have been supplemented by off-center PCs in the OPLS force field to model the anisotropy of the ESP,<sup>7,8</sup> sometimes referred to as ‘extra charge’ or lone pair sites, introduced in the AMBER force field to better describe hydrogen bonding and halogen interactions,<sup>21,22</sup> or virtual interaction sites in GROMACS that can be used for off-center charge models.<sup>23</sup> More generally, the atomic multipole expansion can be approximated using multiple point charges distributed around an atomic center.<sup>24</sup> To obtain a representation of the multipole expansion up to the quadrupole level, six charges per atom are required.<sup>24</sup> Like atomic

multipoles, improvements in interaction energies have also been observed with distributed charge models.<sup>25</sup> The derived multipoles are sensitive to the local atomic environment and therefore exhibit strong conformational dependence<sup>26,27</sup> suggesting that a static representation of atomic multipoles may not be sufficient in some cases. Geometrically dependent distributed charge models have also been considered.<sup>28,29</sup> When modeling the molecular ESP, significant redundancy in electrostatic parameters has been observed.<sup>30</sup> This has justified the use of minimal distributed charges<sup>31</sup> which involved fitting charges to atomic environments and combining these initial guesses using differential evolution (DE) to obtain a model with low complexity and sufficient quality.<sup>31</sup>

In force-field development, it is often desirable to obtain ‘transferable’ parameters across some predefined chemical space whereby topologically similar atoms are assigned the same ‘atom type’ to reduce the complexity of the model.<sup>13,21,25,32</sup> Ideally, these shared parameters should be accurate for molecules not explicitly included during parameterization.<sup>33,34</sup> Transferable multipoles were investigated by Bereau and coworkers<sup>33,34</sup> using predefined reference frames based on handcrafted atom types<sup>26,33</sup> Alternatively, transferability can be obtained without predefined reference frames by using a molecular frame of reference, which can be derived from the principal moments of inertia, where the handedness of the axes system is defined by setting the positive direction of each axis as the vector pointing from a given atom to the molecule’s center of mass.<sup>35,36</sup> Neural networks with directional features can learn a ‘representation’ of local reference frames from the data which may improve transferability.<sup>37</sup> The difference between ‘hand-crafted’ versus learnt local reference frames is analogous to manually constructed features used in Behler–Parrinello atomistic neural networks versus data-driven features learnt by message-passing networks such as PhysNet.<sup>38</sup>

Geometric deep learning<sup>39,40</sup> has emerged as a promising strategy for problems where strong inductive priors stemming from the laws of physics, such as the invariance of energy with respect to rotations and translations, can be leveraged to create efficient, performant, and physically meaningful models.<sup>39,40</sup> Equivariant neural networks are data-efficient, universal

approximators for tasks where inherent symmetries exist, such as rotational equivariance.<sup>41–43</sup> For example, vector quantities such as dipole moments should rotate with the molecule.<sup>35,36</sup> Equivariant neural networks have been applied to the prediction of atomic multipole expansions.<sup>37</sup> By including higher order many-body messages based on spherical harmonics, techniques such as Multiple Atomic Cluster Expansion (MACE),<sup>44</sup> as well as equivariant attention mechanisms,<sup>45</sup> have shown state-of-the-art accuracy in a variety of tasks, such as predicting molecular dipole moments. This approach has also been generalized to Cartesian tensors, which may require fewer parameters.<sup>46</sup> Kernel-based methods using rotationally equivariant features have also been used to model the molecular dipole moment.<sup>47</sup> If only scalar properties are of interest, traditional deep neural networks are sufficient, e.g., for predicting electrostatic parameters for the polarizable Drude classical force field.<sup>48</sup> Although strict equivariant models have garnered significant attention, alternatives which weaken these requirements have been found to provide better performance when large amounts of training data and compute resources are available.<sup>49,50</sup> For instance, the Point Edge Transformer,<sup>49</sup> a graph neural network where each message-passing layer is given by an arbitrarily deep transformer. Furthermore, strategies such as data augmentation<sup>51</sup> have been employed whereby the input and output features are rotated arbitrarily during training.<sup>51</sup> Learning a representation of the density has been explored via construction of the Hamiltonian matrix in a block-wise manner from equivariant representations,<sup>52</sup> as well as grid based electron density learning schemes.<sup>53,54</sup>

Motivated by these examples, we side-step hand-crafted multipole representations to data-driven, symmetry-preserving predictions of off-center charges with a focus on parameterizing the ESP. Here we describe “DCM-net” (distributed charge model network) the first equivariant neural network for the prediction of distributed charges which is trained to minimize the error of the molecular ESP (to our knowledge; related prior work includes equivariant prediction of atomic multipoles and non-equivariant distributed-charge models).<sup>24,28,29,31,37</sup> The model predicts up to  $n_{\text{DC}}$  distributed charges per atom. The performance of the model at reproducing

the ESP and molecular dipole moment is assessed on a hold-out set of unseen structures to assess the model’s transferability.

## 2 Methods

First, a cursory background on molecular electrostatics is presented, then the SO(3)-equivariant architecture is described, along with data curation, training objectives, and various evaluations.

### 2.1 Electrostatics, Multipoles, and Distributed Charges

The electrostatic potential (ESP) at a point  $\mathbf{r}$  arising from a continuous charge distribution  $\rho(\mathbf{r}')$ , omitting the prefactor  $(4\pi\epsilon_0)^{-1}$  for clarity, is

$$\text{ESP}(\mathbf{r}) = \int_{V'} \frac{\rho(\mathbf{r}')}{|\mathbf{r} - \mathbf{r}'|} dV' \quad (1)$$

Expanding the ESP in a Taylor series about a chosen expansion center, typically the center of charge or an atomic nucleus, yields the familiar multipole expansion.<sup>55</sup> In spherical coordinates, and truncated at maximum angular momentum  $\ell_{\text{max}}$ , the ESP

$$\text{ESP}(r, \theta, \phi) \approx \sum_{\ell=0}^{\ell_{\text{max}}} \sum_{m=-\ell}^{\ell} Q_{\ell}^m Y_{\ell}^m(\theta, \phi) R_{\ell}(r) \quad (2)$$

Here,  $Y_{\ell}^m(\theta, \phi)$  are spherical harmonics,  $R_{\ell}(r)$  are radial functions determined by the order of the multipole, and the coefficients  $Q_{\ell}^m$ , the multipole moments, encode the angular components of the charge distribution.<sup>2,55,56</sup> These coefficients can be derived from  $\rho(\mathbf{r}')$ , though they depend on the choice of partitioning scheme when applied to atoms in molecules, and are therefore not unique.<sup>2,27</sup> The lowest-order terms correspond to familiar physical quantities (see Figure 1a;  $\ell = 0$ : monopole (total charge),  $\ell = 1$ : dipole moment,  $\ell = 2$ : quadrupole tensor).

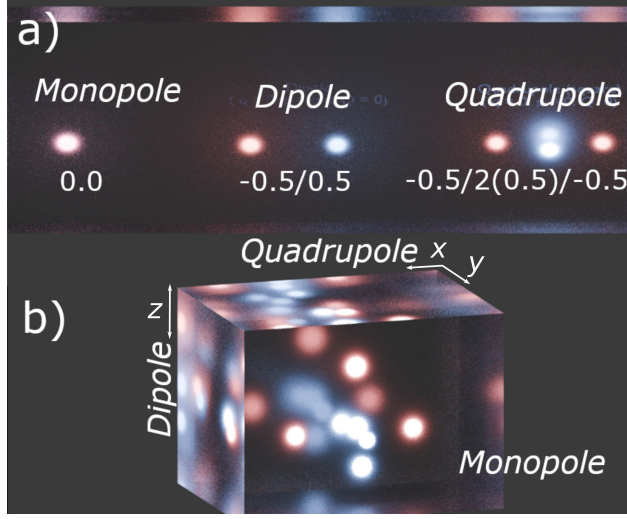

Figure 1: Reproducing the ESP: a graphical illustration of equations 3, 4, and 5 using a computer render of colored ‘point lights’ in glass. a) The standard point charge representations of the monopole, dipole, and quadrupole moments. b) Aligning the dipole in the  $z$  direction and the quadrupole in the  $x$  and  $y$  directions gives a distributed charge solution for a system with vanishing monopole moment (or center of mass or charge). Inside the glass cube, the field may be imprecise (in the chemical problem this can be accepted due to quantum effects such as electronic shielding); however, on the surface, an approximation close to quadrupole order is possible; and distributed charges may be more parameter efficient in certain cases when fitting the field to volumes of interest (such as belt around the van der Waals radii), especially in the case of vanishing molecular (or atomic) multipole moments.

A finite set of symmetrically arranged monopoles can exactly reproduce the low-order multipoles; for example, a system of six judiciously placed charges would be correct up to quadrupole order, defining the monopole (placed at the center of mass), dipole (two charges placed at some coordinates scaled by  $r$ ), and selected quadrupole components (placed at some coordinate scaled by  $r^2$ ).<sup>24,31</sup> In this fashion, the number of charges would scale as  $O((1 + \ell)^2 - \ell + 1)$ . For example, the total charge (referred to here as the ‘monopole’) is

$$Q_0^0 = q = \sum_{i=1}^6 q_i \quad (3)$$

The dipole moments in the  $z$ ,  $x$ , and  $y$  directions (expressed using real spherical harmonic

convention for  $Q_1^m$ ) are

$$Q_1^0 = \mu_z = \sum_{i=1}^6 q_i r_{z,i}, \quad Q_1^{-1} = \mu_x = \sum_{i=1}^6 q_i r_{x,i}, \quad Q_1^1 = \mu_y = \sum_{i=1}^6 q_i r_{y,i} \quad (4)$$

and the (non-redundant) quadrupole terms are

$$Q_2^0 = \Theta_{zz} = \sum_{i=1}^6 \frac{1}{2} q_i (3r_{z,i}^2 - r_i^2), \quad Q_2^{2c} = \frac{1}{\sqrt{3}} (\Theta_{xx} - \Theta_{yy}) = \sum_{i=1}^6 \frac{3}{4} q_i (r_{x,i}^2 - r_{y,i}^2) \quad (5)$$

Here,  $r_{x,i}, r_{y,i}, r_{z,i}$  are the Cartesian coordinates of each point charge  $q_i$  in a local coordinate frame (typically the principal axis system), and  $r_i^2 = r_{x,i}^2 + r_{y,i}^2 + r_{z,i}^2$ . This construction is illustrated in Figure 1 using a computer render of colored ‘point lights’ in glass. The first three moments are reproduced when the dipole moment is aligned in the  $z$  direction, orthogonal to the quadrupole moment in the  $x$  and  $y$  directions. While this example uses six charges to exactly reproduce the leading multipole moments, fewer charges can be used to generate approximate representations of the ESP, giving rise to the minimal distributed charge model (MDCM).<sup>31</sup> The use of distributed point charges in this way underlies the DCM formalism employed in the present work.

This motivates a compact representation of anisotropy via a small set of off-center charges; DCM-net learns their positions and magnitudes from local environments while preserving rotational behavior.<sup>7,8,22</sup>

## 2.2 SO(3)-Equivariant Graph Neural Network

DCM-Net predicts the charge and position of a set of distributed monopoles to represent the molecular electrostatic potential (ESP). It is implemented in JAX<sup>57</sup> using the e3x package.<sup>58</sup> The model employs a message-passing architecture composed of equivariant dense layers and tensor product operations, described below and illustrated in Figure 2. The choice of an

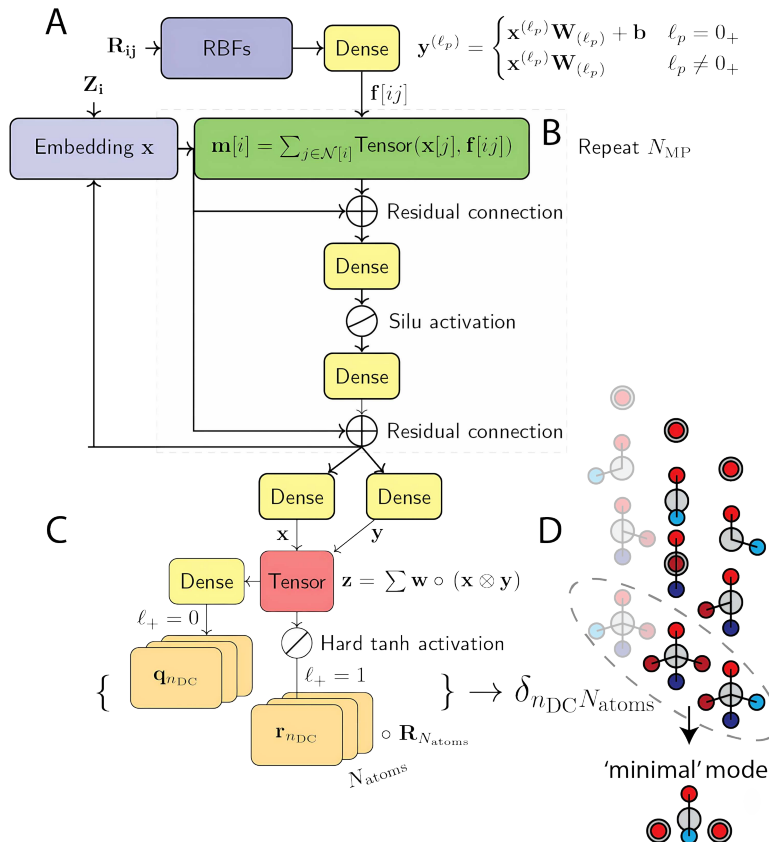

Figure 2: The architecture of DCM-net model. (A) The inputs to the network are atomic numbers and positions expanded into atom-atom distances. (B) During the message passing phase, the hidden representation is updated over  $N_{\text{MP}}$  iterations using the message passing operation (green). Dense layers (Eq. 6) and tensor products (Eq. 7) are shown in yellow and red, respectively. (C) The final output is split between scalar features (monopoles) and vector-like features (charge displacements relative to atomic centers). (D) Predictions using  $n_{\text{dc}}$  distributed charges (red, blue) per atom (gray) can be combined and optimized to create 'minimal' models with acceptable accuracy and improved computational efficiency, and can be used in molecular dynamics simulations.

equivariant architecture is motivated, in the SI, by way of a toy example.

An equivariant dense layer operates analogously to a standard multilayer perceptron when propagating scalar (rotation-invariant) features, with weights  $\mathbf{W}$  and biases  $\mathbf{b}$ . For tensor-valued features (e.g., vector dipoles), the bias term is omitted to preserve  $\text{SO}(3)$  equivariance (see 'Dense layer' in Figure 2A).<sup>41,42</sup> Let  $\ell$  denote the degree of the spherical harmonic (or equivalently, the rank of the irreducible representation), and let  $p = (-1)^\ell$  denote the parity under inversion. The layer transformation is:

$$\mathbf{y}^{(\ell)} = \begin{cases} \mathbf{x}^{(\ell)} \mathbf{W}^{(\ell)} + \mathbf{b}, & \ell = 0 \text{ (scalar)} \\ \mathbf{x}^{(\ell)} \mathbf{W}^{(\ell)}, & \ell > 0 \text{ (tensor)} \end{cases} \quad (6)$$

Tensor features are combined via tensor product operations (denoted "Tensor" in Figure 2), which mix compatible input irreducible representations based on angular momentum coupling rules. The tensor product is parameterized by a learnable weight  $\mathbf{w}_{(l_1, l_2, l_3)}$ , and computes the coupled output features  $\mathbf{z}^{(l_3)}$ :

$$\mathbf{z}^{(l_3)} = \sum_{(l_1, l_2) \in V} \mathbf{w}_{(l_1, l_2, l_3)} \circ (\mathbf{x}^{(l_1)} \otimes^{(l_3)} \mathbf{y}^{(l_2)}) \quad (7)$$

Here, the set  $V$  contains valid combinations of  $(l_1, l_2)$  for a given output  $l_3$ , constrained by the Clebsch–Gordan decomposition rules. Each  $\mathbf{w}_{(l_1, l_2, l_3)} \in \mathbb{R}^{1 \times 1 \times F}$  is a learnable weight shared across features (broadcast over all atoms). The elementwise product  $\circ$  denotes broadcasting over tensor dimensions.

The tensor product  $\otimes^{(l_3)}$  performs coupling of input features using Clebsch–Gordan coefficients<sup>35,36</sup> (Eq. 8):

$$(\mathbf{x}^{(l_1)} \otimes \mathbf{y}^{(l_2)}) m_3^{(l_3)} = \sum m_1 = -l_1^{l_1} \sum_{m_2=-l_2}^{l_2} C_{l_1, l_2, l_3}^{m_1, m_2, m_3}, x_{m_1}^{(l_1)} y_{m_2}^{(l_2)} \quad (8)$$

Here,  $C_{l_1, l_2, l_3}^{m_1, m_2, m_3}$  are the Clebsch–Gordan coefficients that ensure the coupled feature transforms according to the  $l_3$  irreducible representation of  $\text{SO}(3)$ .

Input features  $\mathbf{x} \in \mathbb{R}^{P_1 \times (L_1+1)^2 \times F}$  and  $\mathbf{y} \in \mathbb{R}^{P_2 \times (L_2+1)^2 \times F}$  are indexed over irreducible representation channels  $(L_i + 1)^2$  corresponding to the number of real spherical harmonic components up to angular momentum  $L_i$ . The parity index  $P_i = 2$  if pseudotensors are included, and  $P_i = 1$  otherwise. The output is  $\mathbf{z} \in \mathbb{R}^{P_3 \times (L_3+1)^2 \times F}$ .

Initial atomic embeddings  $\mathbf{x}$  are obtained from atomic numbers  $\mathbf{Z}$  via a learnable embedding layer. Interatomic displacement vectors  $\mathbf{R}_{ij}$  are computed from atom positions and expanded

in a product basis consisting of radial and angular terms:

$$\Phi_{lm}(r, \theta, \phi) = B_n(r)Y_{lm}(\theta, \phi) \quad (9)$$

where  $Y_{lm}$  are real spherical harmonics and  $B_n(r)$  are radial basis functions. Following,<sup>58</sup> Bernstein polynomials for  $B_n(r)$  are used, due to their compact support and ease of enforcing boundary conditions, as a basis with spherical harmonics parameterized by the maximum degree and the number of basis functions. Reciprocal Bernstein radial functions modified by a smooth cutoff function were also included in the features.<sup>58</sup> The standard message passing scheme involves the application of the graph convolution  $\phi_e$  on edge features  $m_{ij}$ , which are summed into node features  $m_i$  used to update the hidden embedding  $h_i$ :

$$m_{ij} = \phi_e(h_i^l, h_j^l, a_{ij}) \quad (10)$$

$$m_i = \sum_{j \in \mathcal{N}(i)} m_{ij} \quad (11)$$

$$h_i^{l+1} = \phi_h(h_i^l, m_i) \quad (12)$$

Each message passing step (Eq. 12) is followed by a dense layer, a SiLU activation function, and finally another dense layer, which is added to the embedding and is repeated for  $n_{\text{MP}}$  steps.

Following the iterative message passing, the atom-wise features undergo further refinement where the output of two dense layers are combined using their tensor product (Eq. 7). The transformation of features to the desired output involves a dense projection to  $n_{\text{DC}}$  per atom. The **hardtanh** activation function scaled by a constant was used to limit the displacements of the distributed charges. The scaling factor used was  $0.175 \text{ \AA}$  to limit displacements to no more than  $0.3 \text{ \AA}$  away from the atomic centers although this hyperparameter may be adjusted.

The displacement of the distributed charges are obtained from the  $\ell_p = 1_-$  features, while

the  $\ell_p = 0_+$  (scalar) features are input into a final dense layer (with an element specific bias) before the final readout step where  $n_{\text{DC}}$  distributed monopoles for each atom are obtained. Here the subscript denotes the parity of the feature, indictating the sign of the feature under inversion (e.g.,  $\ell_p = 1_-$  denotes the odd parity features which change sign under inversion). The final positions of the distributed charges,  $\boldsymbol{\delta}$ , is the sum of the atom’s position  $\mathbf{R}$  and the displacement vector obtained in the final readout  $\mathbf{r}$ .

A physical law, aside from rotational equivariance, enforced by the model is the conservation of charge in an isolated system. The total charge of the molecule,  $Z$ , is constrained by subtracting the mean predicted charge of the total  $N_{\text{DC}}$  charges in the system by the mean total charge:

$$\langle q \rangle = \frac{Z}{N_{\text{atoms}}} - \frac{1}{N_{\text{DC}}} \sum_i^{N_{\text{DC}}} q_i \quad (13)$$

Empirically,<sup>37,41,52</sup> including this constraint has been shown to hinder training, as it likely smooths an already glassy loss landscape, causing the model to become stuck in worse local minima, resulting in slower convergence to typically worse local minima. Penalizing the total molecular charge is more stable and to be preferred. The regularization of Eq. 13 can be applied during inference if required.

The loss function includes terms relating the root-mean-squared error of the electrostatic potential evaluated on the grid,  $\text{RMSE}_{\text{ESP}}$ , between the reference molecular  $\text{ESP}_{\text{ref}}$  obtained from quantum chemical calculations and the ESP from the distributed charges  $\boldsymbol{\delta}$  (a vector consisting of a position and charge) evaluated over  $N_{\text{grid}}$  grid points  $\mathbf{y}_i$ , where the model ESP is calculated as the sum of the Coulomb interactions between each (distributed) charge and a probe charge of  $1e$ .

$$\text{RMSE}_{\text{ESP}}(\boldsymbol{\delta}) := \sqrt{\frac{1}{N_{\text{grid}}} \sum_{i=1}^{N_{\text{grid}}} [\text{ESP}_{\text{ref}}(\mathbf{y}_i) - \text{ESP}_{\text{model}}(\mathbf{y}_i, \boldsymbol{\delta})]^2} \quad (14)$$

An additional (optional) term in the loss function corrects the molecular dipole moment of the distributed charges ( $\mathbf{M}_{\text{DC}}^1 = \sum_{i=0}^{N_{\text{atoms}}} N_{\text{DC}} q_{\text{DC},i}(\mathbf{R}_{\text{CoM}} - \delta_{\text{DC},i})$ ), weighted by  $w_{\text{D}}$  is included in the loss function (Eq. 15):

$$\mathcal{L} = w_{\text{ESP}} \cdot \text{RMSE}_{\text{ESP}} + w_{\text{q}} \cdot \frac{1}{N_{\text{atoms}}} \sum_{i=0}^{N_{\text{atoms}}} \left( M_{\text{ref},i}^0 - \sum_{j=0}^{N_{\text{DC}}} M_{i,j}^0 \right)^2 + w_{\text{D}} \cdot \frac{1}{3} \sum_{\alpha=\{x,y,z\}} (M_{\text{ref},\alpha}^1 - M_{\text{DC},\alpha}^1)^2 \quad (15)$$

The mean absolute error between the MBIS monopoles and the per-atom sum of the distributed charges, weighted by  $w_{\text{q}}$  is also included. This term ensures that the distributed charges are able to reproduce the MBIS monopoles, however, any baseline charge assignment scheme can be used. Regularizing the sum of atomic charges to match the MBIS monopoles is an additional constraint also used in methods

## 2.3 Data Generation

A total of 126900 molecules from QM9<sup>59</sup> were split into three folds of 40000 structures each, and an additional holdout set of 6900 remaining structures was kept for testing. These structures were split based on their order in QM9 (i.e. based on the number of atoms): the training and test set contained molecules with 1 to 8 and 8 to 9 heavy atoms, respectively. QM9 consists of molecules containing carbon, hydrogen, oxygen and fluorine, up to nine heavy atoms. Analysis of the dataset based on the SMILES string deposited in the original QM9 dataset was performed using RDKit<sup>60</sup> (version 2023.5) and TMAP.<sup>61</sup> As is typical when working with QM9,<sup>52,62–64</sup> structures that failed simple consistency checks were removed, namely molecules with energies that were poorly converged or molecules that decomposed during optimization. For a given molecule, the energy was converged at the PBE0/def2-TZVP level of theory using PSI4,<sup>65</sup> and the wavefunction was analyzed, from which MBIS multipoles<sup>18</sup> up to  $\ell = 2$  and the electrostatic potential (evaluated on up to 3200 grid points) were obtained. Grid points were sampled on a regular grid generated by increasing

the bounding box of the molecule by  $\pm 3.0 \text{ \AA}$  along every direction, sampling 15 points along each axis. As the electrostatic potential distorts close to atomic nuclei due to charge penetration effects, a careful selection of grid points is important. Different grid point sampling methods were explored: an element-independent minimum distance cutoff of  $1.7 \text{ \AA}$  (i.e., one times the vdW radius of the largest atom, i.e., carbon), and element-dependent minimum distance cutoffs of 1.4 times the vdW radii. Due to this sampling scheme, larger molecules typically had lower density of grid points. Alternative examples of training data with mixed radial and angular grids were also explored. Specifically, the same grids as used in the RESP method were tested, *post-hoc* and not used in any data in the main manuscript; however, the performance was seemingly improved, based on the quality of the dipole moment prediction. These observations are analogous to the long-range Coulomb interaction problem, which (famously) converges differently depending on how the long-range interaction pairs are selected.<sup>66</sup>

## 2.4 Model and Training Details

The DCM-net models were configured with the following hyperparameters: two message passing iterations, a cutoff radius of  $4.0 \text{ \AA}$  (used to define graph edges), and a feature size of 16, and 8 radial basis functions, respectively. Optimization of the NN was performed using the ADAM optimizer<sup>67</sup> ( $\beta_1 = 0.9$ ,  $\beta_2 = 0.999$ ,  $\epsilon = 10^{-8}$ ) as implemented in the Optax library,<sup>57</sup> with a batch size of one. The loss function (Eq. 15) was weighted to balance the ESP and charge predictions. Specifically, the weight on the electrostatic potential term,  $w_{\text{ESP}} = 10^5$ , preserves the original Hartree/ $e$  units. This choice resulted in ESP and dipole contributions of comparable magnitude during training, when the weight for the atomic charges was  $w_q = 1.0$ . Initial experiments used an exponentially decaying learning rate (from  $1 \cdot 10^{-3}$  to  $1 \cdot 10^{-5}$ ) and gradient clipping (global norm, clip norm = 1),<sup>68</sup> with the objective of minimizing the squared error in the MBIS-derived monopoles and ESP (see Eq. 15). Learning curves from these models were used to validate the implementation (more details

are provided in the SI). This weighting term was typically 1-2 orders of magnitude larger for the ESP than the total charge and molecular dipole terms. Charge weights  $w_q = 1.0$  ensured a correct first moment of the ESP to within 0.001 electron charge units, although training on datasets containing molecules with a non-zero net charge may require larger weights. Data were split into three non-overlapping training/validation sets based on the order of molecules in the GDB dataset.<sup>69</sup> This introduced a sampling bias due to the underlying graph enumeration algorithm, leading to chemically similar structures within individual splits.

Training set sizes of 8k, 16k, and 32k molecules were used to benchmark and, in particular, learning curves, each with a constant validation set size of 8k structures. These models were trained for 500 epochs with a batch size of 16 and a learning rate of  $1 \cdot 10^{-4}$ . Final models were trained on 64k structures for 1000 epochs, using an 8k validation set and 6.9k molecules held out for testing. Molecular similarity was evaluated using the Tanimoto coefficient computed in RDKit,<sup>60</sup> based on two-hop Morgan fingerprints (1024 bits). TMAP projections<sup>61</sup> were generated using the MHFP encoder<sup>70</sup> to visualize molecular space coverage.

## 2.5 Experiments, Analysis, and Refinement

Additional transfer learning experiments were performed outside the scope of the QM9 dataset which is restricted to equilibrium structures. Here, coordinates of 2040 random, neutral dipeptides sampled from gas-phase MD simulations at 500 K using were obtained from the SPICE dataset described by Eastman and coworkers.<sup>71</sup> Calculations as described above were performed to obtain the ESPs and molecular dipole moments. All alanine and glycine dipeptides (63 conformers) were deposited in the test set. This prevents any indirect data leakage and helps justify the transferability of this approach. The remaining structures were used in the training and validation sets (1900 and 77, respectively).

DCM-net predicts a fixed number of distributed charges per atom; however, these predictions

can be combined or filtered to improve or adapt the charge model. In this work, hydrogen atoms were assigned only an atom-centered monopole, while heavy atoms received either one or more distributed charges based on either a fixed total number of charges per molecule, or the anisotropy of the ESP around the atom, as estimated from the dipole or traceless quadrupole tensor norm(s). Once the distributed charges were selected, the total molecular charge was corrected via charge equilibration as described in Eq. 13. This adaptive charge assignment strategy was compared to a global optimization method based on differential evolution.<sup>31</sup>

To assess robustness beyond the training setup, we evaluate under a finer ESP grid and a different level of theory. To evaluate the model’s ability to extrapolate, ESP predictions were compared to a roughly ten-fold finer reference ESP grid than was used during training. The grid was partitioned into close- ( $1.20 < r < 1.66$ ) , mid- ( $1.66 < r < 2.20$ ) , and far-range ( $2.20 < r$ ) regions relative to the molecular surface (see Table 1). Additionally, this reference ESP data was computed at a different level of theory (MP2/6-31G(d,p)) using Gaussian16,<sup>72</sup> in contrast to the DFT-level ESPs used for training. This ensures a fair assessment of the transferability of the approach across different levels of theory, which is critical when employing these models in force-field fitting to alternative reference data.

### 3 Results and Discussion

We evaluate DCM-net along three axes: (1) practical generation of minimal charge models, (2) ESP accuracy versus MBIS multipoles, and (3) transfer learning to out-of-distribution dataset of dipeptides. First, we demonstrate the model’s ability to generate minimal distributed charges which can readily be applied to MD simulations in packages such as CHARMM.<sup>73</sup> As illustrated in Figure 3, the predicted charge displacements and ESP evaluations transform consistently under rotations of the inputs. Following this, an analysis of the accuracy of the

model is provided in comparison to density derived atomistic multipole expansions obtained from MBIS, as well as a discussion on the training dynamics and model validation using the learning curves. Finally, the capability for applying these models in a transfer learning setting is investigated.

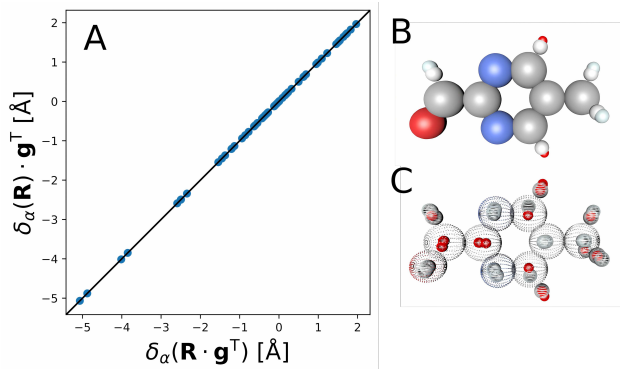

Figure 3: (A) Cartesian components of the predicted distributed charge positions  $\delta$  (shown in B and C) transform equivariantly with respect to the input atomic positions  $\mathbf{R}$  after a rotation  $\mathbf{g}$  is applied. Similarly, rotating the grid points and evaluating the ESP provide identical predictions.

### 3.1 Generating Minimal Distributed Charge Models

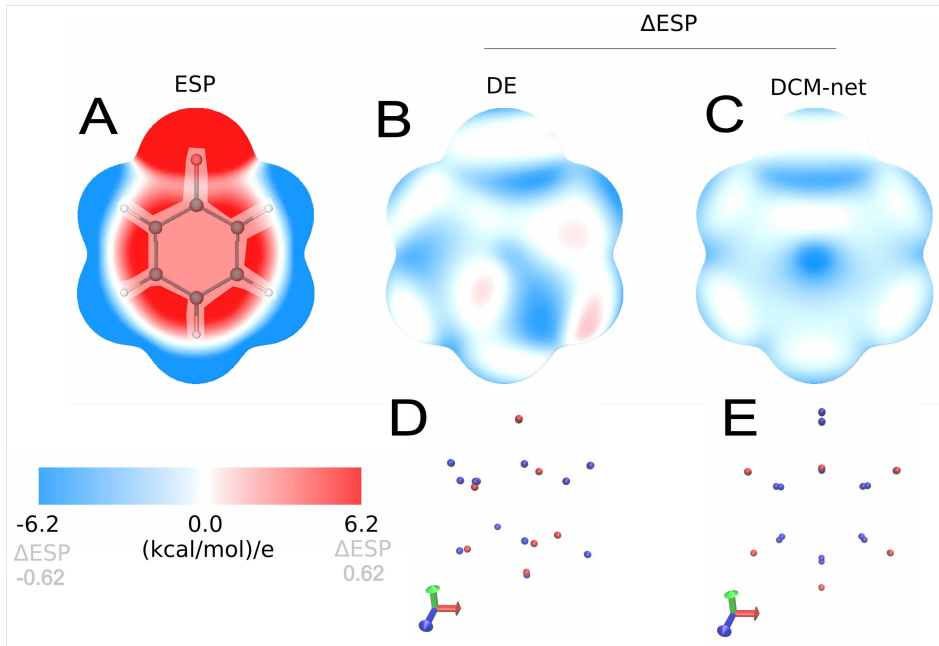

Figure 4: The ground truth electrostatic potential surface of fluorobenzene using a color map from -6.2 to (6.2 kcal/mol)/e, at an isodensity of 0.01 a.u., compared to the error surfaces from a 19 charge model generated by differential evolution (DE) and DCM-net (two-charge-per-heavy-atom), using a color map from -0.62 to 0.62 (10% of the original colorbar). Both models achieve similar accuracy (0.6 versus 0.5 (kcal/mol)/e), despite no fitting being used for the DCM-net prediction. The error surface of the equivariant model is consistent with the symmetry of the molecule.

The model’s ability to generate “minimal” distributed charge models was investigated. Fluorobenzene (Figure 4) was selected for this task, as the molecule was not included in the training set but is still within the data distribution of QM9 (i.e.  $< 10$  heavy atoms). The results are compared with a model obtained using a differential-evolution optimization scheme<sup>31</sup> where 19 charges were selected as a viable trade-off between complexity and accuracy. Having established that DCM-net produces symmetry-consistent minimal models comparable to DE, we next quantify ESP accuracy against multipolar baselines. In this case, two charges per heavy atom were assigned from the two-charge DCM-net model, while hydrogen atoms were assigned on-site charges determined by the one-charge model. The model obtained from DCM-net was similar or slightly better than the model obtained from DE for all regions of

Table 1: Comparison of RMSE, Max Error, and Number of Points for two sets of data across different ranges. The grid points are selected based on  $r$ , the ratio of the distance divided by the vdW radii for the closest atom.

| <b>Range</b>                    | <b>DCM-net</b>      |      | <b>DE</b>           |      | $N_{\text{grid}}$ |
|---------------------------------|---------------------|------|---------------------|------|-------------------|
|                                 | RMSE <sub>ESP</sub> | max. | RMSE <sub>ESP</sub> | max. |                   |
| Total                           | 5.4e-01             | 12.8 | 6.2e-01             | 12.9 | 415153            |
| Close ( $1.20 < r < 1.66$ )     | 1.1                 | 12.8 | 1.2                 | 12.9 | 90064             |
| Mid-range ( $1.66 < r < 2.20$ ) | 2.3e-01             | 1.4  | 3.3e-01             | 1.5  | 152428            |
| Far-range ( $2.20 < r$ )        | 7.5e-02             | 0.4  | 1.1e-01             | 0.6  | 172661            |

the ESP, including maximum errors (Table 1).

Since the DCM-net model leverages the symmetry of the local molecular environment, the distributions of errors across the ESP surface are essentially symmetric. In contrast, if the grid points selected are not symmetric, which can occur if too few grid points are chosen, the symmetry of the optimized model will be broken. It is also possible to enforce symmetric charge positions based on the entire point group of the molecule; however, such high symmetry examples become less common for larger molecules. Leveraging the local symmetries of the atomic environments is clearly advantageous, as it leads to similar distributed charge positions for similar functional groups, without any requirements on the molecule global symmetry, and can smoothly interpolate between similar molecules/conformations. To summarize, meaningful proposals for distributed charges can be generated in seconds rather than hours of CPU hours for the DE routine. Given these advantages, a practical application of this model is in automated force field and topology builders.<sup>23,73–76</sup>

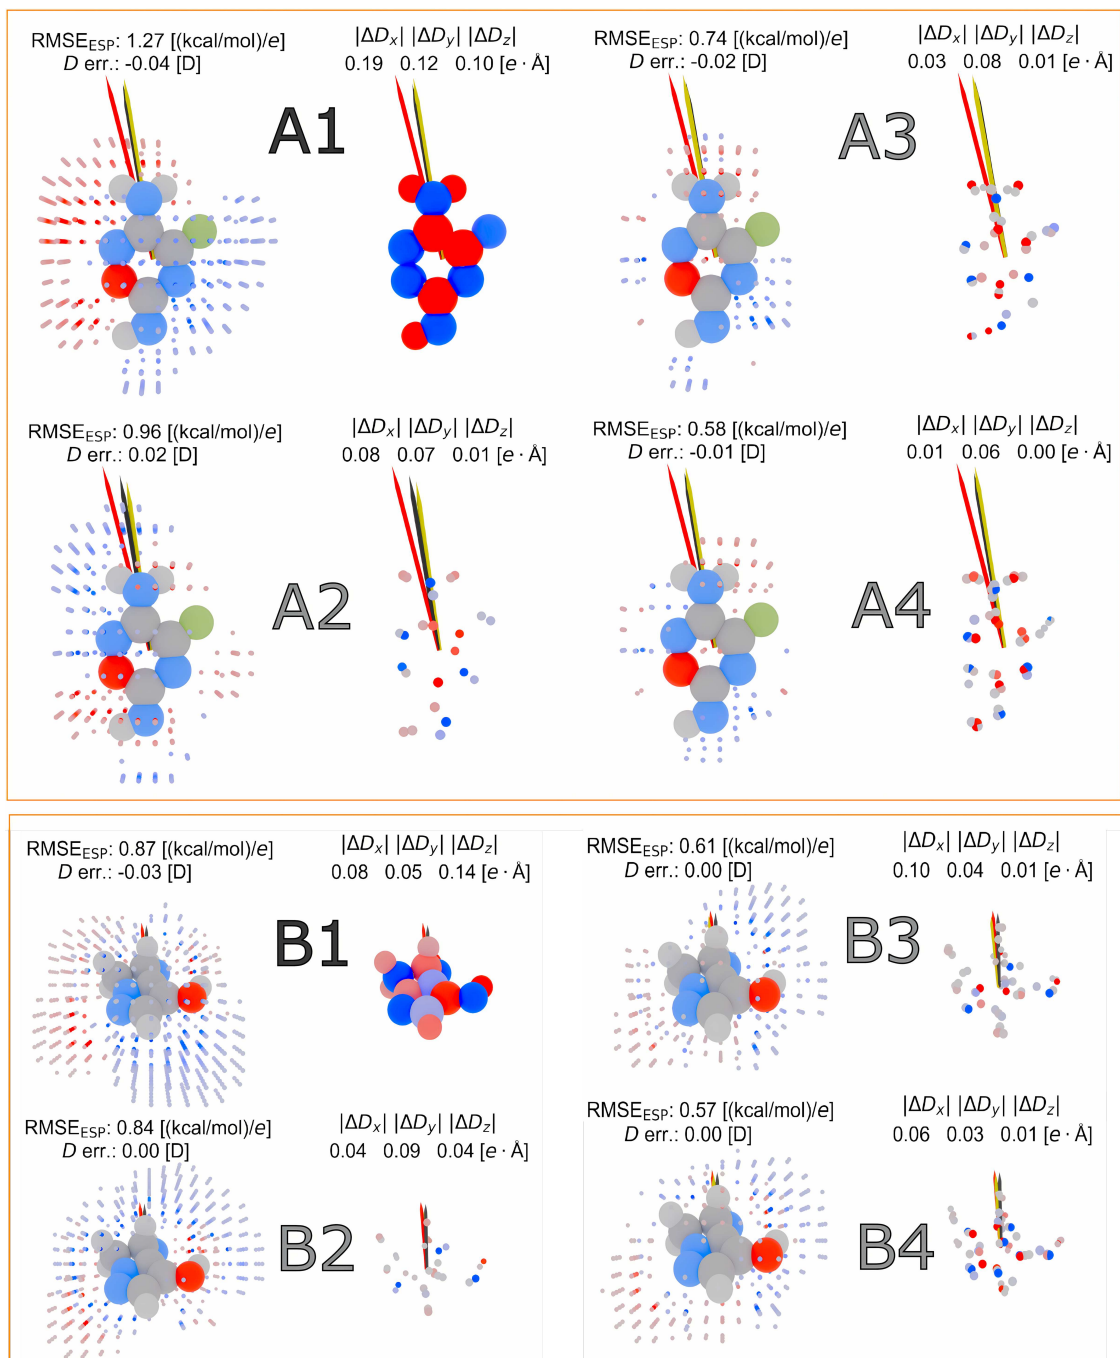

Figure 5: The spatial extent of the improvement introduced by DCM-net in comparison to MBIS point charges (note the colorscale is qualitative; identifying regions of positive/negative errors and charge), for ‘cherry-picked’ test set examples A and B, with (1) MBIS point charges, (2) two-, (3) three-, and (4) four-charge-per-atom DCM-net predictions. On the left, grid points with greater than 75% of the absolute error for the monopole ESP. On the right, molecular dipole vectors (scaled by  $4\times$  for clarity) of (black) the ground truth, and of (red) the MBIS monopole and (yellow) DCM-net models. Errors, typically, decrease as the number of distributed charges per atom increases.

### 3.2 Accuracy of the Electrostatic Potential

The distributed charge positions predicted by DCM-net are able to reduce the average RMSE error in the ESP in comparison to fitted MBIS monopoles, and reach similar accuracy of the fitted multipole expansion up to  $l = 1$  when more than two-charges-per-atom are predicted (Table 2); however, the accuracy for the four-charges-per-atom model is slightly worse than the MBIS expansion up to atomic quadrupoles (0.6 versus 0.5 (kcal/mol)/ $e$  on the test set). Figure 6A reports the distribution of ESP errors for increasing multipole ranks/number of distributed charges per atom for all molecules in the test set. The shape of the error distributions for multipole- and distributed charge-based ESPs are comparable, indicating a uniform improvement for the test set as the number of distributed charges increases. If the error distributions associated with the predicted distributed charges were skewed with heavy tails it may suggest that the learned distributed charge representations were biased towards certain types of molecules; however, the similar improvements in the error distributions suggest the DCM-net approach is transferable (at least within the chemical space of QM9) and increasing the number of distributed charges provides benefits almost on par with increasing the rank of the multipole expansion.

The sum of the distributed charges per atom closely matches the target MBIS monopoles (Table 2) implying that the improvement is a result of the anisotropic nature of the off-center charges and not due to the model ‘cheating’ by assigning physically unrealistic charges to buried atoms, as mentioned earlier. This assessment is further supported by comparing the distributions of such charges obtained using MBIS and DCM-net, as well as a general fixed charge force field such as CGenFF (see SI, Figure S5). By applying this constraint, predictions from DCM-net can be converted to an equivalent atom-centered model on an atom-by-atom basis to create minimal models with acceptable accuracy and low computational complexity.

Figure 5 shows examples of the positions of the predicted distributed charges, as well as

points of the error surface with errors higher than 75% of the absolute errors obtained with fitted atom-centered point charges. Due to the nature of the problem, i.e. the inverse square law, the error is expected to be larger at closer distances from the atom, so grid points further away from the molecule show regions where the anisotropic potential contains significant errors.<sup>55</sup> Strikingly, all distributed charge models are able to reduce the error of grid points around the fluorine atom (shown in green, Figure 5A2-A4), which is expected to have pronounced anisotropic features in the ESP due to the  $\sigma$ -hole effects that are known to be difficult to capture with atom centered point charges alone.<sup>6-8</sup> The location of grid points have implications seen in the predicted charge magnitudes. For instance, when the models were trained on grid points closer than 1.4 times the van der Waals radii of the atoms (i.e. points where the potential is heavily influenced by charge penetration effects), although the DCM-net models had lower overall RMSEs than the MBIS-fitted point charges, the spatial distributions of grid points with high errors were typically larger demonstrating a bias towards close-range points of the ESP. When this issue in the training data was addressed, i.e. by excluding close range point, the spatial distributions of errors were more similar to the MBIS-fitted point charges without any drawbacks to the overall accuracy of the ESP.

To understand where anisotropic charges help most, we break down each grid point ESP errors into categories: (1) by the closest element, and (2) by the closest atom type in the CGenFF force field. Although the potential at a certain grid point is based on contributions from the entire molecule, the closest atom/distributed charge is expected to have the largest impact on the associated error. Additionally, since atoms such as carbon are usually occluded by hydrogen atoms, the relative orientation of the grid points assessed using this approach will be different for different atom types, so the relative errors for different elements cannot be compared directly, although a comparison between different electrostatic models using this approach is consistent.<sup>2,77</sup> For atom-centered multipoles, the average quality of the ESP around carbon and nitrogen atoms is only significantly improved with the addition of atom

centered quadrupoles as many heteroaromatic rings present in the test set are expected to have significant quadrupole contributions to the ESP stemming from the presence of  $\pi$ .<sup>2,14</sup> In contrast, distributed charges appear to be an efficient way of representing such anisotropic charge distributions as even the two-charge-per-atom model reaches quadrupole accuracy around these atomic centers.

For fluorine, the improvement gained from more than two-charges-per-atom is much smaller in comparison to increasing the rank of the multipole expansion. In contrast, the addition of atomistic quadrupoles nearly halves the median  $\text{RMSE}_{\text{ESP}}$ . For oxygen atoms, the addition of atom centered dipoles correspond to a 0.5 reduction in the median  $\text{RMSE}_{\text{ESP}}$  (from  $\sim 1.1$  to  $\sim 0.6$  (kcal/mol)/ $e$ ), which is related to the improved description of hydroxy (-OH) groups which have a significant dipole character.

The improvement gained by including two-distributed-charges-per-atom instead is slightly smaller (from  $\sim 1.1$  to  $\sim 0.8$  (kcal/mol)/ $e$ ) approximating the dipole quality when three-distributed-charges-per-atom are included ( $\sim 0.6$  (kcal/mol)/ $e$ ) but only slight improvements are gained when increasing the representation to a four-distributed-charges-per-atom model. The same analysis was repeated by separating the grid points into a larger number of classes based on their proximity to different CGenFF atom types (see SI, S1 and S2). Here, only molecules in the test set with valid CGenFF atom types were analysed and the amount of data for each class is significantly lower and considering the limitations mentioned above it is more difficult to make well-grounded conclusions as to which atom types benefit the most from improved electrostatic representations. As expected, increasing the rank of the MBIS multipole expansion monotonically decreases the errors associated with all atom types (Table S1). In contrast, using this ad-hoc partitioning scheme reveals that the learnt distributed charge representations only provide a small improvement in comparison to MBIS monopoles for certain atom types and, furthermore, the improvement gain from increasing the number

of distributed charges per atom is not monotonic in all cases likely due to the stochastic nature of training and the non-unique nature of the fitting problem resulting in a glassy loss landscape. Unsurprisingly, given the chemical diversity of the four splits in the SI (Figure S3), chemical biases were observed in training.

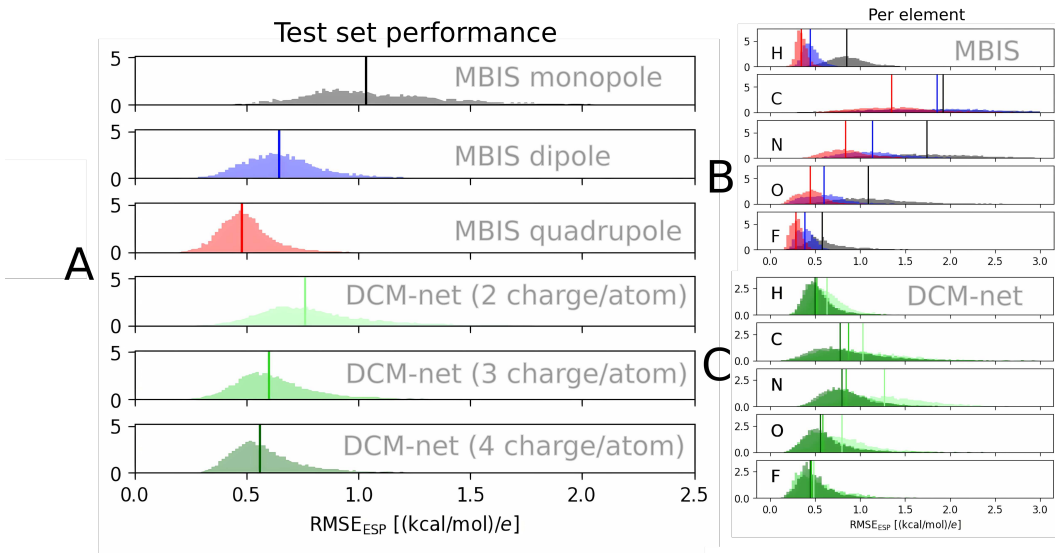

Figure 6: (A) Distribution of  $\text{RMSE}_{\text{ESP}}$  values (difference between the model and reference ESP) for the entire hold-out (test) set, (B) contributions based on individual elements contributions for multipoles and (C) DCM-net. The normalized probability density is shown on the  $y$ -axis. Atom centered multipole expansions up to monopole (black), dipole (blue) and quadrupole (red) are shown along with the two-, three-, and four-charge-per atom models shown in pale green, green and dark green, respectively. The median of the distributions are shown with vertical lines. Note the change in height of the distributions for the DCM-net models due to fatter tails in the distribution.

As for all deep-learning models, performance drops are expected when leaving the training distribution.<sup>78–80</sup> One limitation of the machine learnt distributed charges is the presence of outliers in the form of long-tails of the distribution. For some structures, the error in the ESP is significantly larger than that of the equivalent MBIS monopoles. An important consideration in the extrapolation capability of atomistic neural network models is the coverage of chemical space in the training data space<sup>78,79</sup> (see SI, Figure S3). The maximum Tanimoto similarity<sup>81</sup> of the 100 structures with highest error in the test was 0.4; compared to 0.5 for 100 structures with

Table 2: Performance of the DCM-net models with  $n_{\text{DC}}$  distributed charges per atom, measured by  $\text{RMSE}_{\text{ESP}}$  error with respect to the reference ESP, in comparison to MBIS multipoles. The average RMSE of the ESP for the molecules in the test set  $\langle \text{RMSE}_{\text{ESP}} \rangle$  values are in (kcal/mol)/ $e$ . The mean absolute error between the sum of the DCM-net distributed charges per atom and MBIS  $\text{MAE}_{l=0}$ ,  $\text{MAE}_{l=0}$ , is in elementary charge  $e$ , and the mean absolute error of the components of the molecular dipole moment,  $\text{MAE}_D$ , is given in Debye.

|                   | $\langle \text{RMSE}_{\text{ESP}} \rangle$ | $\text{MAE}_{l=0}$ | $\text{MAE}_D$ |
|-------------------|--------------------------------------------|--------------------|----------------|
| $l = 0$           | 1.1                                        | -                  | 0.195          |
| $l \leq 1$        | 0.7                                        | -                  | 0.001          |
| $l \leq 2$        | 0.5                                        | -                  | 0.001          |
| $n_{\text{DC}}=2$ | 0.8                                        | 4.0e-02            | 0.123          |
| $n_{\text{DC}}=3$ | 0.7                                        | 3.2e-02            | 0.110          |
| $n_{\text{DC}}=4$ | 0.6                                        | 3.0e-02            | 0.105          |

the lowest errors, which suggests that these outliers may be related to insufficient training examples for particular types of molecules.

### 3.3 Reproducing the Molecular Dipole Moment with Distributed Charges

The mean absolute errors of the components of the molecular dipole moment for various models is given in Table 2. Although the two-charge-per-atom model significantly reduces the error in the molecular dipole moment in comparison to MBIS monopoles (from 0.195 D to 0.123 D), the improvement saturates with increasing numbers of distributed charges per atom with the three and four charge models exhibiting only slight improvements (0.110 D and 0.105 D). These results are inline with previous atom centered point charge models such as PhysNet;<sup>38</sup> however, still behind that of atom centred multipoles<sup>37</sup> and naturally behind the performance of MBIS atomistic dipoles derived from wavefunction based densities so naturally fit the data better.<sup>18</sup> In contrast, the MBIS atomistic dipoles are, by construction, functions of local atomic densities and are fit to reproduce the total dipole of the molecular wavefunction and as a result the associated errors are small (0.001 D). A significant advantage is that unlike the simulated dipole produced by two off-center point charges, atom centered

dipoles can simply be added together to obtain the molecular dipole moment since the two are both rank-1 tensors. Distributed charges behave like monopoles (rank-0 tensors) and finding a solution that best represents the ESP while also reproducing the molecular dipole moment is therefore more challenging.<sup>39</sup> It is important to emphasize the general message that choosing a model with the appropriate prior, i.e. using atomistic dipoles (popularized by Anthony Stone<sup>27</sup>) to represent molecular dipoles, will usually lead to more accurate predictions. In general, non-equilibrium conformations improved the accuracy of the molecular dipole moment, , and any sufficiently large dataset capturing variations of geometry, and therefore variations in wavefunction and ESP, can be thought of regularizing the fitting problem similar to conformational averaging of charge models<sup>28,29</sup> (although operating on local chemical environments rather than the entire molecular reference frame) and is also a regularization technique used commonly in machine learning potentials.<sup>64</sup>

### 3.4 Transfer Learning

Finally, we test generalization to flexible, protein-like motifs by adapting the model to a dipeptide set via lightweight transfer learning. Transfer learning exploits mutual information between different tasks to speed-up training and to increase performance in downstream (usually orthogonal) tasks.<sup>82,83</sup> Here, we investigate transfer learning predictions of the model based on QM-minimized structures to structures obtained from cruder molecular mechanics-based methods. Training on structures from QM9 introduce a bias to (near) equilibrium conformations which make the predictions of the model sensitive to the level of theory of the geometry optimization.<sup>59,63</sup> One simple test carried out was to take the SMILES representation of the molecule and recalculate the molecular geometry using RDKit’s standard (empirical) distance-geometry-based conformer generator.<sup>60</sup> These structures were typically tens of kcal/mol higher in energy than the geometries obtained from QM9, and contain molecules with substantially different distributions of bond lengths and angles present in QM9.

In this out-of-distribution regime, the ESP errors were generally worse than that of the fitted MBIS monopoles. These are not deficits of the model per se, since the data set can be adapted and the model can be retrained using a transfer learning strategy.<sup>82,83</sup> As in previous studies,<sup>82,83</sup> the learning rate was decreased by a factor of 100 to 2.5e-07, and all parameters of the model were optimised over 1000 steps of transfer learning. The final average ESP error over the unseen structures was 0.6 (kcal/mol)/ $e$ , constituting a 0.2 (kcal/mol)/ $e$  improvement over the MBIS monopoles (0.8 (kcal/mol)/ $e$ ); and the MAE of the molecular dipole was 0.1314 D in comparison to 0.2552 D.

Modest improvements in comparison to fitted MBIS monopoles are consistent with the results in Table 2, and suggest that the two-charge-per-atom model is not competitive with higher order multipolar expansions derived from atomic densities (bear in mind these are fit to reproduce the first three moments of the ESP), as the inclusion of atomistic dipoles with and without quadrupoles achieved 0.4 and 0.3 (kcal/mol)/ $e$  in the average RMSE of the ESP, and reached a MAE of 0.002 D across predictions of the molecular dipole moment. The weaker results on the dipole moment are due to (1) approximation errors due to using point charges (instead of atomistic dipoles) and (2) difficulties in training with multiple objectives and constraints in the loss function. Training iteratively between putting higher weights on either the dipole or ESP objectives, improved the final results slightly, as is observed when training models on energy and forces.<sup>58</sup> These improvements were modest and not included in the results presented in this paper to give a fairer sense of the performance of the model, although empirically this approach is recommended. For a premium solution, training a molecular dipole surface, in combination with distributed charges for a well described local ESP, alongside a NN force field for local interactions would be an appealing compromise for modelling small molecules. During transfer learning, the observed decrease in required training time and increase in accuracy constitute additional evidence that the features learned by the model are robust and transferable to different molecular conformations or chemical systems.

## 4 Conclusions

Across tasks, DCM-net produces symmetry-consistent minimal models quickly and reduces ESP error relative to fitted MBIS monopoles, approaching dipole-level multipolar accuracy when two or more charges per atom are used, particular in regions with  $\pi$  bonds and  $\sigma$ -hole effects. Equivariance through construction, as presented here, is ultimately a design choice and alternatives such as data augmentation are routinely employed.<sup>39,49</sup> Such as in this setting, where evaluation of the Coulomb potential grid can become costly in memory and compute, the data efficiency of EGNNs is advantageous.<sup>84</sup> The approach outlined in this paper streamlines the generation of distributed charge with specified accuracy or complexity. These models can be introduced as rigid distributed point charges into empirical force fields and given a diverse training set, additional parameters can be optimized against a consistent charge model in a transferable fashion, allowing for the rapid development of force fields with anisotropic electrostatics.

## Acknowledgement

This work was supported by the Swiss National Science Foundation through grants 200020\_219779 and 200021\_215088 and the University of Basel.

## Supporting Information Available

All data and computer codes for this work are available from the authors upon request as well as core functionality for building the training dataset, as well as training and evaluating the model being available from the public repository at <https://github.com/EricBoittier/dcmnet>. Additionally, figures made using Blender 4.3 (Figures 1 and 5) can be obtained there. A demo of the model is available as a Space on HuggingFace at <https://huggingface.co/spaces/EricBoi/DCM-net>. Future developments, as well as

hands-on tutorials for FF parameterization and QM/MM calculations will be made available from a parent repository at <https://github.com/EricBoittier/mmml.git>.

## References

- (1) Bayly, C. I.; Cieplak, P.; Cornell, W.; Kollman, P. A. A well-behaved electrostatic potential based method using charge restraints for deriving atomic charges: the RESP model. *J. Phys. Chem.* **1993**, *97*, 10269–10280.
- (2) Stone, A. J. *The Theory of Intermolecular Forces*, 2nd ed.; Oxford University Press, 2013.
- (3) Murray, J. S.; Politzer, P. The Electrostatic Potential: An Overview. *WIREs Comput. Mol. Sci.* **2011**, *1*, 153–163.
- (4) Politzer, P.; Murray, J. S. The Fundamental Nature and Role of the Electrostatic Potential in Atoms and Molecules. *Theor. Chem. Acc.* **2002**, *108*, 134–142.
- (5) Suresh, C. H.; Remya, G. S.; Anjalikrishna, P. K. Molecular Electrostatic Potential Analysis: A Powerful Tool to Interpret and Predict Chemical Reactivity. *WIREs Comput. Mol. Sci.* **2022**, *12*, e1601.
- (6) Ibrahim, M. A. A. Molecular mechanical study of halogen bonding in drug discovery. *J. Chem. Theory Comput.* **2011**, *32*, 2564–2574.
- (7) Jorgensen, W. L.; Schyman, P. Treatment of halogen bonding in the OPLS-AA force field: application to potent anti-HIV agents. *J. Chem. Theory Comput.* **2012**, *8*, 3895–3901.
- (8) Yan, X. C.; Robertson, M. J.; Tirado-Rives, J.; Jorgensen, W. L. Improved Description of Sulfur Charge Anisotropy in OPLS Force Fields: Model Development and Parameterization. *J. Phys. Chem. B* **2017**, *121*, 6626–6636.

- (9) Kolář, M.; Hobza, P. On Extension of the Current Biomolecular Empirical Force Field for the Description of Halogen Bonds. *J. Chem. Theory Comput.* **2012**, *8*, 1325–1333.
- (10) Kramer, C.; Spinn, A.; Liedl, K. R. Charge Anisotropy: Where Atomic Multipoles Matter Most. *J. Chem. Theory Comput.* **2014**, *10*, 4488–4496.
- (11) Faerman, C. H.; Price, S. L. A transferable distributed multipole model for the electrostatic interactions of peptides and amides. *J. Am. Chem. Soc.* **1990**, *112*, 4915–4926.
- (12) Plattner, N.; Meuwly, M. The role of higher CO-multipole moments in understanding the dynamics of photodissociated carbonmonoxide in myoglobin. *Biophys. J.* **2008**, *94*, 2505–2515.
- (13) Ponder, J. W.; Wu, C.; Ren, P.; Pande, V. S.; Chodera, J. D.; Schnieders, M. J.; Haque, I. et al. Current status of the AMOEBA polarizable force field. *J. Phys. Chem. B* **2010**, *114*, 2549–2564.
- (14) Day, G. M.; Motherwell, W. D. S.; Jones, W. Beyond the Isotropic Atom Model in Crystal Structure Prediction of Rigid Molecules: Atomic Multipoles versus Point Charges. *Cryst. Growth Des.* **2005**, *5*, 1023–1033.
- (15) Devereux, M.; Gresh, N.; Piquemal, J.-P.; Meuwly, M. A supervised fitting approach to force field parametrization with application to the SIBFA polarizable force field. *J. Comput. Chem.* **2014**, *35*, 1577–1591.
- (16) Dykstra, C. E. Electrostatic Interaction Potentials in Molecular Force Fields. *Chem. Rev.* **1993**, *93*, 2339–2353.
- (17) Heindel, J. P.; Kim, L.; Head-Gordon, M.; Head-Gordon, T. Completely Multipolar Model for Many-Body Water–Ion and Ion–Ion Interactions. *J. Phys. Chem. Lett.* **2025**, *16*, 975–984.

- (18) Verstraelen, T.; Vandenbrande, S.; Heidar-Zadeh, F.; Vanduyfhuys, L.; Van Speybroeck, V.; Waroquier, M.; Ayers, P. W. Minimal Basis Iterative Stockholder: Atoms in Molecules for Force-Field Development. *J. Chem. Theory Comput.* **2016**, *12*, 3894–3912.
- (19) Smith, D. G. A.; Lolincio, A. T.; Glick, Z. L.; Lee, J.; Alenaizan, A.; Barnes, T. A.; Borca, C. H. et al. Quantum Chemistry Common Driver and Databases (QCDB) and Quantum Chemistry Engine (QCE NGINE ): Automation and Interoperability among Computational Chemistry Programs. *J. Chem. Phys.* **2021**, *155*, 204801.
- (20) Misquitta, A. J.; Stone, A. J.; Fazeli, F. Distributed Multipoles from a Robust Basis-Space Implementation of the Iterated Stockholder Atoms Procedure. *J. Chem. Theory Comput.* **2014**, *10*, 5405–5418.
- (21) Weiner, S. J.; Kollman, P. A.; Case, D. A.; Singh, U. C.; Ghio, C.; Alagona, G.; Profeta, S. et al. A new force field for molecular mechanical simulation of nucleic acids and proteins. *J. Am. Chem. Soc.* **1984**, *106*, 765–784.
- (22) Dixon, R. W.; Kollman, P. A. Advancing beyond the atom-centered model in additive and nonadditive molecular mechanics. *J. Comput. Chem.* **1997**, *18*, 1632–1646.
- (23) Abraham, M.; Alekseenko, A.; Basov, V.; Bergh, C.; Briand, E.; Brown, A.; Doijade, M. et al. GROMACS 2024.2 Manual. 2024; <https://doi.org/10.5281/zenodo.11148638>.
- (24) Devereux, M.; Raghunathan, S.; Fedorov, D. G.; Meuwly, M. A Novel, Computationally Efficient Multipolar Model Employing Distributed Charges for Molecular Dynamics Simulations. *J. Chem. Theory Comput.* **2014**, *10*, 4229–4241.
- (25) Devereux, M.; Boittier, E. D.; Meuwly, M. Systematic improvement of empirical energy functions in the era of machine learning. *J. Comput. Chem.* **2024**, *45*, 1899–1913.
- (26) Kramer, C.; Gedeck, P.; Meuwly, M. Atomic multipoles: Electrostatic potential fit, local

- reference axis systems, and conformational dependence. *J. Comput. Chem.* **2012**, *33*, 1673–1688.
- (27) Koch, U.; Popelier, P.; Stone, A. Conformational dependence of atomic multipole moments. *Chem. Phys. Lett.* **1995**, *238*, 253–260.
- (28) Boittier, E. D.; Devereux, M.; Meuwly, M. Molecular Dynamics with Conformationally Dependent, Distributed Charges. *J. Chem. Theory Comput.* **2022**, *18*, 7544–7554.
- (29) Boittier, E.; Töpfer, K.; Devereux, M.; Meuwly, M. Kernel-based Minimal Distributed Charges: A Conformationally Dependent ESP-Model for Molecular Simulations. **2024**, arXiv:2406.00513 [physics].
- (30) Jakobsen, S.; Jensen, F. Systematic Improvement of Potential-Derived Atomic Multipoles and Redundancy of the Electrostatic Parameter Space. *J. Chem. Theory Comput.* **2014**, *10*, 5493–5504.
- (31) Unke, O. T.; Devereux, M.; Meuwly, M. Minimal distributed charges: Multipolar quality at the cost of point charge electrostatics. *J. Chem. Phys.* **2017**, *147*, 161712.
- (32) Warshel, A.; Kato, M.; Pisiakov, A. V. Polarizable Force Fields: History, Test Cases, and Prospects. *J. Chem. Theory Comput.* **2007**, *3*, 2034–2045.
- (33) Bereau, T.; Kramer, C.; Meuwly, M. Leveraging Symmetries of Static Atomic Multipole Electrostatics in Molecular Dynamics Simulations. *J. Chem. Theory Comput.* **2013**, *9*, 5450–5459.
- (34) Bereau, T.; Andrienko, D.; von Lilienfeld, O. A. Transferable Atomic Multipole Machine Learning Models for Small Organic Molecules. *J. Chem. Theory Comput.* **2015**, *11*, 3225–3233.
- (35) Zare, R. N. *Angular Momentum: Understanding Spatial Aspects in Chemistry and Physics*; John Wiley & Sons, 1988.

- (36) Brink, D. M.; Satchler, G. R. *Angular Momentum*, 3rd ed.; Oxford University Press, 1993.
- (37) Thürlemann, M.; Bösel, L.; Riniker, S. Learning Atomic Multipoles: Prediction of the Electrostatic Potential with Equivariant Graph Neural Networks. *J. Chem. Theory Comput.* **2022**, *18*, 1701–1710.
- (38) Unke, O. T.; Meuwly, M. PhysNet: A Neural Network for Predicting Energies, Forces, Dipole Moments, and Partial Charges. *J. Chem. Theory Comput.* **2019**, *15*, 3678–3693.
- (39) Bronstein, M. M.; Bruna, J.; LeCun, Y.; Szlam, A.; Vandergheynst, P. Geometric deep learning: going beyond Euclidean data. *IEEE Signal Process. Mag.* **2017**, *34*, 18–42, arXiv:1611.08097 [cs].
- (40) Duval, A.; Mathis, S. V.; Joshi, C. K.; Schmidt, V.; Miret, S.; Malliaros, F. D.; Cohen, T. et al. A Hitchhiker’s Guide to Geometric GNNs for 3D Atomic Systems. **2024**, arXiv:2312.07511 [cs, q-bio, stat].
- (41) Schütt, K.; Unke, O.; Gastegger, M. Equivariant message passing for the prediction of tensorial properties and molecular spectra. Proceedings of the 38th International Conference on Machine Learning. 2021; p 9377–9388.
- (42) Batatia, I.; Batzner, S.; Kovács, D. P.; Musaelian, A.; Simm, G. N. C.; Drautz, R.; Ortner, C. et al. The Design Space of E(3)-Equivariant Atom-Centered Interatomic Potentials. **2022**, arXiv:2205.06643 [cond-mat, physics:physics, stat].
- (43) Brandstetter, J.; Hesselink, R.; van der Pol, E.; Bekkers, E. J.; Welling, M. Geometric and Physical Quantities Improve E(3) Equivariant Message Passing. **2022**, arXiv:2110.02905 [cs, stat].
- (44) Batatia, I.; Kovács, D. P.; Simm, G. N. C.; Ortner, C.; Csányi, G. MACE: Higher Order

- Equivariant Message Passing Neural Networks for Fast and Accurate Force Fields. **2023**, arXiv:2206.07697 [cond-mat, physics:physics, stat].
- (45) Frank, J. T.; Unke, O. T. So3krates: Equivariant attention for interactions on arbitrary length-scales in molecular systems. **2023**, arXiv:2205.14276 [cond-mat, physics:physics].
  - (46) Simeon, G.; de Fabritiis, G. TensorNet: Cartesian Tensor Representations for Efficient Learning of Molecular Potentials. **2023**, arXiv:2306.06482 [physics].
  - (47) Sun, J.; Cheng, L.; Miller, I., Thomas F. Molecular dipole moment learning via rotationally equivariant derivative kernels in molecular-orbital-based machine learning. *J. Chem. Phys.* **2022**, *157*, 104109.
  - (48) Kumar, A.; Pandey, P.; Chatterjee, P.; MacKerell, A. D. Deep Neural Network Model to Predict the Electrostatic Parameters in the Polarizable Classical Drude Oscillator Force Field. *J. Chem. Theory Comput.* **2022**, *18*, 1711–1725.
  - (49) Pozdnyakov, S. N.; Ceriotti, M. Smooth, exact rotational symmetrization for deep learning on point clouds. **2023**, arXiv:2305.19302 [cond-mat, physics:physics].
  - (50) Wang, Y.; Elhag, A. A.; Jaitly, N.; Susskind, J. M.; Bautista, M. A. Swallowing the Bitter Pill: Simplified Scalable Conformer Generation. **2024**,
  - (51) Glick, Z. L.; Koutsoukas, A.; Cheney, D. L.; Sherrill, C. D. Cartesian message passing neural networks for directional properties: Fast and transferable atomic multipoles. *J. Chem. Phys.* **2021**, *154*, 224103.
  - (52) Unke, O.; Bogojeski, M.; Gastegger, M.; Geiger, M.; Smidt, T.; Müller, K.-R. SE(3)-equivariant prediction of molecular wavefunctions and electronic densities. Advances in Neural Information Processing Systems. 2021; p 14434–14447.
  - (53) Koker, T.; Quigley, K.; Taw, E.; Tibbetts, K.; Li, L. Higher-order equivariant neural networks for charge density prediction in materials. *npj Comput. Mater.* **2024**, *10*, 1–10.

- (54) Li, C.; Sharir, O.; Yuan, S.; Chan, G. K. Image Super-resolution Inspired Electron Density Prediction. **2024**, arXiv:2402.12335 [physics].
- (55) Jackson, J. D. *Classical electrodynamics*, 3rd ed.; John Wiley & Sons, 1999.
- (56) Buckingham, A. D.; Disch, R. L.; Dunmur, D. A. Quadrupole Moments of Some Simple Molecules. *J. Am. Chem. Soc.* **1968**, *90*, 3104–3107.
- (57) Babuschkin, I.; Baumli, K.; Bell, A.; Bhupatiraju, S.; Bruce, J.; Buchlovsky, P.; Budden, D. et al. The DeepMind JAX Ecosystem. 2020; <http://github.com/google-deepmind>.
- (58) Unke, O. T.; Maennel, H. E3x: E(3)-Equivariant Deep Learning Made Easy. **2024**, arXiv:2401.07595 [physics].
- (59) Ramakrishnan, R.; Dral, P. O.; Rupp, M.; von Lilienfeld, O. A. Quantum chemistry structures and properties of 134 kilo molecules. *Sci. Data* **2014**, *1*, 140022.
- (60) Landrum, G.; Tosco, P.; Kelley, B.; Ric,; Cosgrove, D.; sriniker,; Vianello, R. et al. rdkit/rdkit: Release\_2023.09.5. 2024; <https://doi.org/10.5281/zenodo.10633624>.
- (61) Probst, D.; Reymond, J.-L. Visualization of very large high-dimensional data sets as minimum spanning trees. *J. Chem. Inf. Model.* **2020**, *12*, 12.
- (62) Unke, O. T.; Meuwly, M. A reactive, scalable, and transferable model for molecular energies from a neural network approach based on local information. *J. Chem. Phys.* **2018**, *148*, 241708.
- (63) Kim, H.; Park, J. Y.; Choi, S. Energy refinement and analysis of structures in the QM9 database via a highly accurate quantum chemical method. *Sci. Data* **2019**, *6*, 109.
- (64) Weinreich, J.; Browning, N. J.; von Lilienfeld, O. A. Machine learning of free energies in chemical compound space using ensemble representations: Reaching experimental uncertainty for solvation. *J. Chem. Phys.* **2021**, *154*, 134113.

- (65) Smith, D. G. A.; Burns, L. A.; Simmonett, A. C.; Parrish, R. M.; Schieber, M. C.; Galvelis, R.; Kraus, P. et al. PSI4 1.4: Open-source software for high-throughput quantum chemistry. *J. Chem. Phys.* **2020**, *152*, 184108.
- (66) Kolafa, J.; Perram, J. W. Cutoff Errors in the Ewald Summation Formulae for Point Charge Systems. **1992**, *9*, 351–368.
- (67) Kingma, D. P.; Ba, J. Adam: A Method for Stochastic Optimization. **2017**,
- (68) Pascanu, R.; Mikolov, T.; Bengio, Y. On the difficulty of training Recurrent Neural Networks. **2013**,
- (69) Ruddigkeit, L.; van Deursen, R.; Blum, L. C.; Reymond, J.-L. Enumeration of 166 Billion Organic Small Molecules in the Chemical Universe Database GDB-17. *J. Chem. Inf. Model.* **2012**, *52*, 2864–2875.
- (70) Probst, D.; Reymond, J.-L. A probabilistic molecular fingerprint for big data settings. *J. Cheminf.* **2018**, *10*, 66.
- (71) Eastman, P.; Behara, P. K.; Dotson, D. L.; Galvelis, R.; Herr, J. E.; Horton, J. T.; Mao, Y. et al. SPICE, A Dataset of Drug-like Molecules and Peptides for Training Machine Learning Potentials. *Sci. Data* **2023**, *10*, 11.
- (72) Frisch, M. J.; Trucks, G. W.; Schlegel, H. B.; Scuseria, G. E.; Robb, M. A.; Cheeseman, J. R.; Scalmani, G. et al. Gaussian~16 Revision C.01. 2016; Gaussian Inc. Wallingford CT.
- (73) Hwang, W.; Austin, S. L.; Blondel, A.; Boittier, E. D.; Boresch, S.; Buck, M.; Buckner, J. et al. CHARMM at 45: Enhancements in Accessibility, Functionality, and Speed. *J. Phys. Chem. B* **2024**, *128*, 9976–10042.
- (74) Stroet, M.; Caron, B.; Visscher, K. M.; Geerke, D. P.; Malde, A. K.; Mark, A. E.

- Automated Topology Builder Version 3.0: Prediction of Solvation Free Enthalpies in Water and Hexane. *J. Chem. Theory Comput.* **2018**, *14*, 5834–5845.
- (75) Kong, L.; Park, S.-J.; Im, W. CHARMM-GUI PDB Reader and Manipulator: Covalent Ligand Modeling and Simulation. *J. Mol. Biol.* **2024**, *436*, 168554.
- (76) Feng, S.; Park, S.; Choi, Y. K.; Im, W. CHARMM-GUI Membrane Builder: Past, Current, and Future Developments and Applications. *J. Chem. Theory Comput.* **2023**, *19*, 2161–2185.
- (77) Wang, B.; Truhlar, D. G. Partial Atomic Charges and Screened Charge Models of the Electrostatic Potential. *J. Chem. Theory Comput.* **2012**, *8*, 1989–1998.
- (78) Vazquez-Salazar, L. I.; Boittier, E. D.; Unke, O. T.; Meuwly, M. Impact of the Characteristics of Quantum Chemical Databases on Machine Learning Prediction of Tautomerization Energies. *J. Chem. Theory Comput.* **2021**, *17*, 4769–4785.
- (79) Itza Vazquez-Salazar, L.; D. Boittier, E.; Meuwly, M. Uncertainty quantification for predictions of atomistic neural networks. *Chem. Sci.* **2022**, *13*, 13068–13084.
- (80) Yang, Z.; Huang, T.; Pan, L.; Wang, J.; Wang, L.; Ding, J.; Xiao, J. QuanDB: A Quantum Chemical Property Database towards Enhancing 3D Molecular Representation Learning. *J. Cheminf.* **2024**, *16*, 48.
- (81) Tanimoto, T. T. *An Elementary Mathematical Theory of Classification and Prediction*; Technical Report, 1958; IBM Internal Technical Report.
- (82) Käser, S.; Boittier, E. D.; Upadhyay, M.; Meuwly, M. Transfer Learning to CCSD(T): Accurate Anharmonic Frequencies from Machine Learning Models. *J. Chem. Theory Comput.* **2021**, *17*, 3687–3699.

- (83) Käser, S.; Richardson, J. O.; Meuwly, M. Transfer Learning for Affordable and High-Quality Tunneling Splittings from Instanton Calculations. *J. Chem. Theory Comput.* **2022**, *18*, 6840–6850.
- (84) Batzner, S.; Musaelian, A.; Sun, L.; Geiger, M.; Mailoa, J. P.; Kornbluth, M.; Molinari, N. et al. E(3)-Equivariant Graph Neural Networks for Data-Efficient and Accurate Interatomic Potentials. *Nature* **2022**, *13*, 2453, arXiv:2101.03164 [cond-mat, physics:physics].

## TOC Graphic

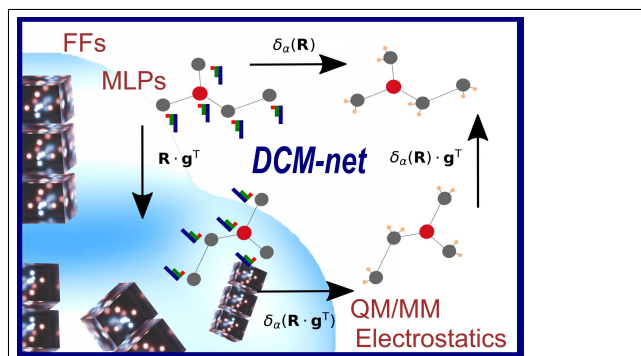

# Supporting Information: Fast, Equivariant Predictions of Distributed Charge Models

Eric D. Boittier and Markus Meuwly\*

*Department of Chemistry, University of Basel, Klingelbergstrasse 80 , CH-4056 Basel, Switzerland.*

E-mail: m.meuwly@unibas.ch

## S1 Why Equivariance?

The advantage of equivariance is motivated with a simplified example, working in 3D space.<sup>1</sup> Consider a regression task aimed at predicting a set of scaled vectors pointing to the center of mass of three points (Fig. S1A). Here, a non equivariant three-layer feed-forward network with a hidden feature size of 21 and a two-layer equivariant network with a feature size of 3 are trained on points positioned in the  $xy$ -plane (Fig. S1). A validation set is constructed where the points can take arbitrary positions in 3D space. The standard neural network is unable to generalize to the validation set (Fig. S1B) because it hasn't seen these rotated examples. In an ENN, the inputs in the training and validation sets are equivalent (albeit rotated) so the test and validation accuracy is comparable, and considerably lower than the standard NN in this toy example.<sup>2,3</sup> Visualizing the hidden states of these networks provides some intuition to this different behavior (Figure S2). If the input  $X$  is permuted via a transpose to  $X^T$  (which corresponds to a valid rotation) the expected output  $Y$  should also be permuted to  $Y^T$ . However, the learned weight matrices of the NN are not permuted causing the output to be incorrect (Figure S2A). In the equivariant example, if all  $l = 1$

features of the input, hidden states, and output are visualized, the states of the neural network appear equivalent for  $X$  and  $X^T$  and only differ by transposition (Figure S2B). If data augmentation is applied by randomly rotating examples, the standard neural network is able to learn this simple function eventually; however, more data and longer training times are usually required to achieve results on par with ENNs.<sup>4</sup> Although this example is extremely contrived, it is common for quantum chemistry software to rotate a molecule to a ‘standard orientation’ (aligned to the principal axes of inertia) so such biases illustrated in the training/validation curves in Fig. S1A) may be introduced if data augmentation is not applied.<sup>5</sup>

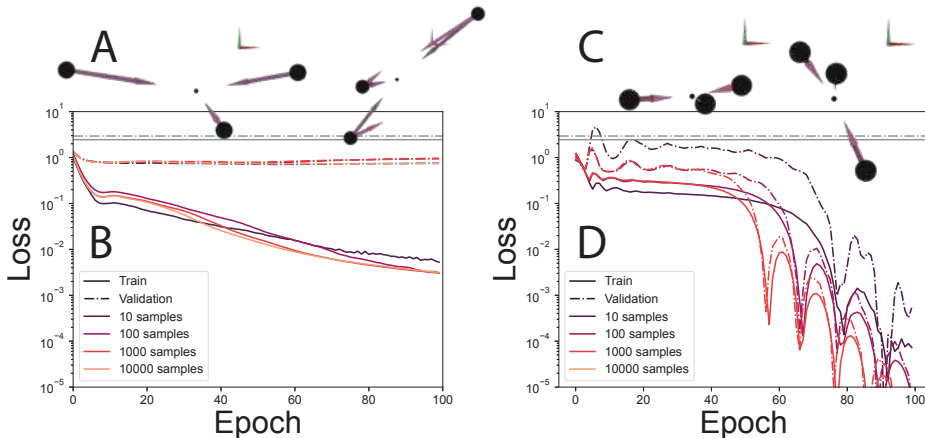

Figure S1: (A) Consider a simplified setting where the task is to predict atom-centered vectors pointing to the center of mass. (B) A feedforward neural network shown examples exclusively in the  $xy$ -plane is unable to generalize if a random rotation is applied to the validation set. (C) Prediction errors from equivariant neural networks (ENNs) are agnostic to global orientation. (D) As a result, ENNs can be more accurate and sample efficient when data is limited or training is costly.

Considering the training loss (solid lines in Figures S1B and D), both NNs perform comparably although the ENN reaches considerably lower values. However, for the validation set (dashed lines), the non-ENN is unable to reach comparably low loss values whereas for the ENN the loss on training and validation sets is comparable. Visualising the hidden states of these networks provides some intuition to this different behaviour (Figure S2). If the input  $X$  is permuted via a transpose to  $X^T$  (which corresponds to a valid rotation) the expected

output  $Y$  should also be permuted to  $Y^T$ . However, the learned weight matrices of the NN are not permuted causing the output to be incorrect (Figure S2A). In the equivariant example, if all  $l = 1$  features of the input, hidden states, and output are visualized, the states of the neural network appear equivalent for  $X$  and  $X^T$  and only differ by transposition (Figure S2B). If data augmentation is applied by randomly translating examples, the standard neural network is able to learn this simple function eventually; however, more data and longer training times are usually required to achieve results on par with ENNs. If data augmentation is restrictive, for example due to training times, biases illustrated in the training/validation curves in Fig. S1A). In other words, using equivariant NNs may be a data reduction strategy.

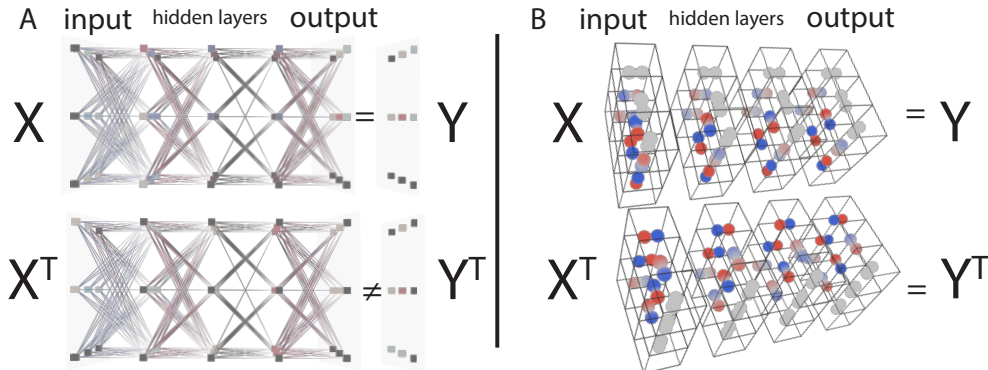

Figure S2: The input, hidden state, and output of a three-layer fully connected network with nodes and edges/weights colored by value for a NN (A) and (B) an ENN (only the  $\ell_p = 1$ -features are depicted and the weights, i.e. coupling paths, are not shown for clarity). If the input  $X$  and output  $Y$  is transposed, the NN prediction is incorrect because the weights are insensitive to this transformation. For the ENN, since all operations are equivariant, the hidden states and output are equivalently transposed when shown  $X$  and  $X^T$ .

## S2 Training Dynamics and Learning Curves

After initialization and even after the first training epoch, the predicted displacement vectors of the distributed charges have approximately zero magnitude, resulting in atom-centered charges. Atom centered charges are equivariant by definition and are a local minimum for

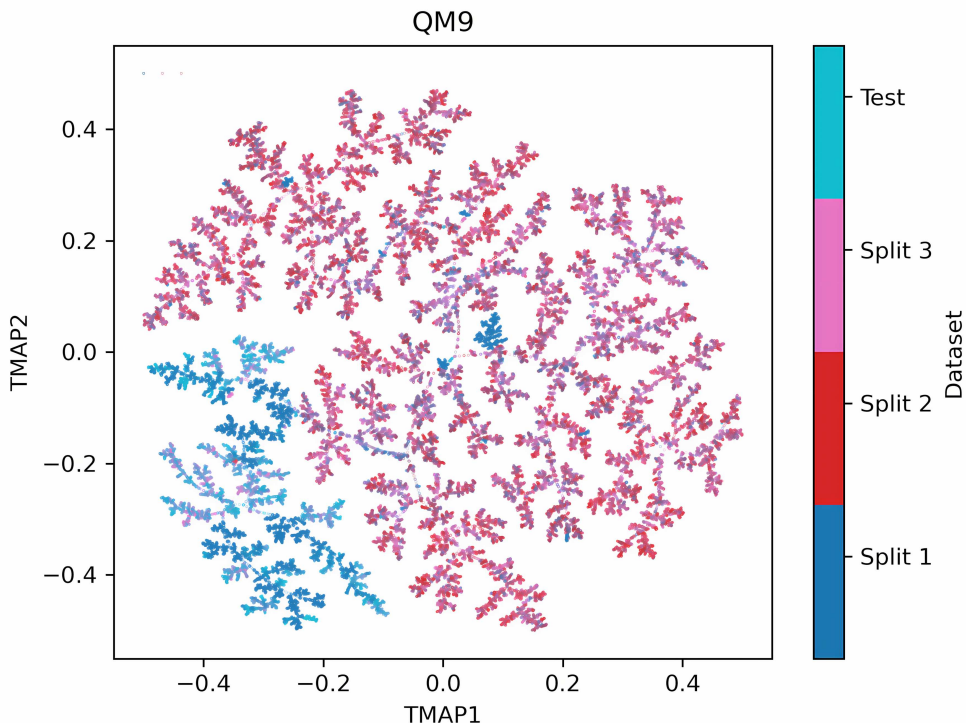

Figure S3: TMAP projection of the dataset colored by split. Learning curves were generated from training on Splits 1 to 3 separately. Final models used all samples from Splits 1 - 3 in the training/validation splits. The test set contains atoms with either 8 or 9 heavy atoms. As observed in previous studies,<sup>6</sup> splitting by the order of the dataset introduces a sampling bias.

the model. To elaborate, finding suitable displacements that generalize across the training set is difficult and atom centered solutions are a simple way to reduce the loss function early on during training. It was observed that, when using gradient clipping, constraining charge displacements and a small learning rate, it was possible to trap the models in this ‘atom-centered local minimum’ regime and subsequently converge the models to an accuracy on par with MBIS monopoles. However, by restarting training without gradient clipping or constraints on charge displacements, the models were able explore true distributed charge solutions and escape such local minima, after which the training could be restarted again with the original protocol.

An important approach in validating new approaches in deep learning is to verify the im-

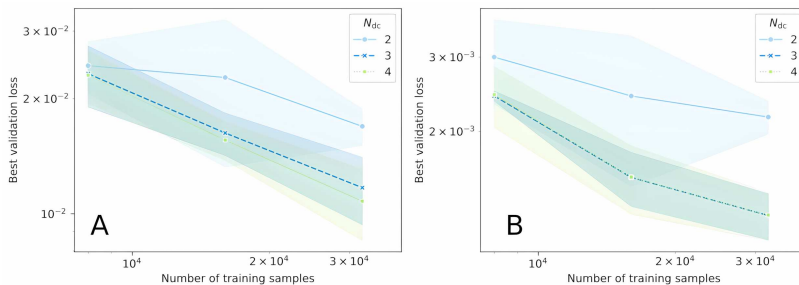

Figure S4: Learning curves for shorter training runs (500 epochs) with an ESP weight  $w$  of  $10^4$  (A) and  $10^3$  (B) using three non-overlapping splits of the data. Shaded areas report the standard deviation for three splits of the training data.

provement of a model given more data. According to statistical learning theory, a model should become more accurate when shown increasing amounts of data.<sup>7</sup> Empirically,<sup>8</sup> this process exhibits a power-law relationship between the size of the data set and the accuracy of the model, which is also this case with DCM-net (Figure S4). The slope of the learning curves for models trained with  $w_{\text{ESP}}$  of  $10^3$  and  $10^4$  are consistent when this prefactor is accounted for. This indicates that fitting to the ESP grid is a viable strategy for obtaining transferable distributed charge models. The variance in the learning curves is significant (Figure S4) due in part to the fact the models were trained on non-overlapping splits. The similar scaling performance observed for 3 and 4 charge models may be related to insufficient training, as the models were not fully converged after 500 epochs. The two charge models showed comparable validation loss with that of the three and four charge models in the low data regime ( $<20\text{k}$  training samples) which demonstrates the variance in the performance of the models. This observation reinforces the point that finding a set of distributed charges that reproduces the ESP is non-unique.

## S3 Training Data Distributions and Chemistry

Following on from the main text, more details on the training data distributions and chemistry are provided. Figure S5 shows the distribution of point charges for the test set using MBIS (black), CGenFF (gold), and DCMNet (green). The distribution of charges for the DCMNet model is similar to that of MBIS, indicating that the model is able to learn the correct charges for the test set.

Table S1 shows the average  $\text{RMSE}_{\text{ESP}}$  ((kcal/mol)/ $e$ ) evaluated on grid points grouped by proximity to the nearest CGenFF atom type using fitted MBIS multipole expansions. Errors less than 0.5 (kcal/mol)/ $e$  are shown in bold. The average  $\text{RMSE}_{\text{ESP}}$  for the DCMNet model is similar to that of MBIS, indicating that the model is able to learn the correct charges for the test set.

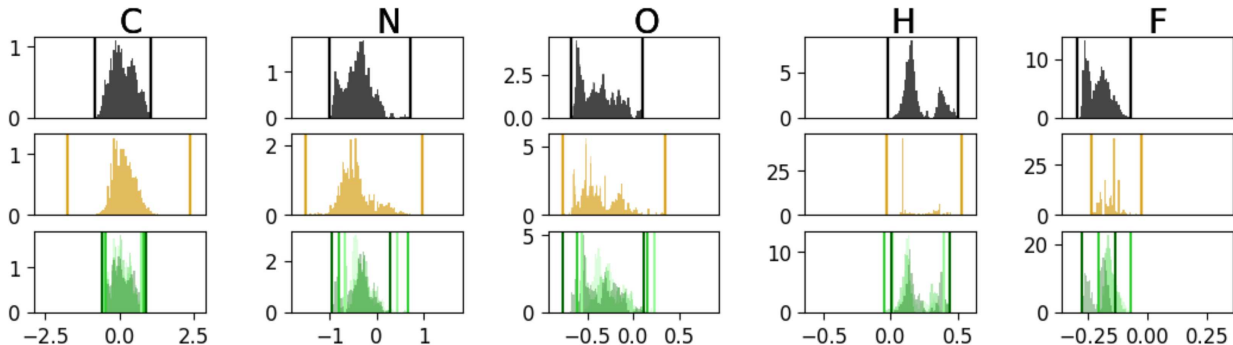

Figure S5: Distribution of point charges for the test set using MBIS (black), CGenFF (gold), and DCMNet (green).

Table S1: The average  $\text{RMSE}_{\text{ESP}}$  ((kcal/mol)/ $e$ ) evaluated on grid points grouped by proximity to the nearest CGenFF atom type using fitted MBIS multipole expansions. Errors less than 0.5 (kcal/mol)/ $e$  are shown in bold.

|        | $l = 0$     | $l \leq 1$  | $l \leq 2$  | description                                                       |
|--------|-------------|-------------|-------------|-------------------------------------------------------------------|
| CG1N1  | 1.34        | 0.71        | <b>0.48</b> | Carbon in cyano group                                             |
| CG1T1  | 1.42        | 0.61        | <b>0.42</b> | Alkyne carbon (R-C)                                               |
| CG1T2  | 0.84        | <b>0.38</b> | <b>0.25</b> | Alkyne carbon (H-C)                                               |
| CG2R71 | 2.59        | 0.64        | <b>0.42</b> | 7-membered aromatic carbon                                        |
| FGA3   | <b>0.20</b> | <b>0.06</b> | <b>0.04</b> | Aliphatic fluorine, trifluoro group                               |
| FGR1   | <b>0.50</b> | <b>0.16</b> | <b>0.10</b> | Aromatic fluorine                                                 |
| HGA1   | <b>0.50</b> | <b>0.12</b> | <b>0.08</b> | Aliphatic proton, CH                                              |
| HGA2   | <b>0.40</b> | <b>0.11</b> | <b>0.07</b> | Aliphatic proton, CH2                                             |
| HGA3   | <b>0.31</b> | <b>0.09</b> | <b>0.06</b> | Aliphatic proton, CH3                                             |
| HGP1   | <b>0.49</b> | <b>0.12</b> | <b>0.08</b> | Polar hydrogen                                                    |
| HGP4   | <b>0.43</b> | <b>0.09</b> | <b>0.06</b> | Polar hydrogen, neutral conjugated -NH2 group                     |
| HGPAM1 | <b>0.49</b> | <b>0.17</b> | <b>0.11</b> | Polar hydrogen, neutral dimethylamine group                       |
| HGPAM2 | <b>0.37</b> | <b>0.08</b> | <b>0.05</b> | Polar hydrogen, neutral methylamine group                         |
| HGR51  | <b>0.47</b> | <b>0.12</b> | <b>0.08</b> | Nonpolar hydrogen, neutral 5-membered planar ring carbon          |
| HGR52  | <b>0.47</b> | <b>0.13</b> | <b>0.09</b> | Aldehyde hydrogen, formamide hydrogen (RCOH)                      |
| HGR61  | <b>0.45</b> | <b>0.16</b> | <b>0.11</b> | Aromatic hydrogen                                                 |
| HGR62  | <b>0.50</b> | <b>0.16</b> | <b>0.11</b> | Nonpolar hydrogen, neutral 6-membered planar ring                 |
| NG1T1  | <b>0.31</b> | <b>0.18</b> | <b>0.12</b> | Nitrogen in cyano group                                           |
| NG2D1  | 1.09        | <b>0.29</b> | <b>0.20</b> | Nitrogen in neutral imine                                         |
| NG2R50 | 0.66        | <b>0.16</b> | <b>0.11</b> | Double-bonded nitrogen in neutral 5-membered planar ring          |
| NG2R60 | 0.79        | <b>0.27</b> | <b>0.18</b> | Double-bonded nitrogen in neutral 6-membered planar ring          |
| NG2R62 | 0.77        | <b>0.22</b> | <b>0.15</b> | Double-bonded nitrogen in 6-membered planar ring with heteroatoms |
| NG321  | 1.76        | <b>0.37</b> | <b>0.26</b> | Neutral methylamine nitrogen                                      |
| OG2D1  | 0.56        | <b>0.16</b> | <b>0.11</b> | Carbonyl oxygen                                                   |
| OG2D4  | 0.72        | <b>0.17</b> | <b>0.12</b> | 6-membered aromatic carbonyl oxygen                               |
| OG2R50 | 0.76        | <b>0.19</b> | <b>0.13</b> | Oxygen in furan ring                                              |
| OG301  | 1.49        | <b>0.37</b> | <b>0.25</b> | Ether oxygen (-O-)                                                |
| OG311  | 0.84        | <b>0.18</b> | <b>0.12</b> | Hydroxyl oxygen                                                   |
| OG3R60 | 1.01        | <b>0.31</b> | <b>0.21</b> | Oxygen in 6-membered cyclic enol, ether, or ester                 |

Table S2: The average  $\text{RMSE}_{\text{ESP}}$  ((kcal/mol)/e) evaluated on grid points grouped by proximity to the nearest CGenFF atom type using trained DCMNet models with the best performance on the training set. Errors less than 0.5 (kcal/mol)/e are shown in bold.

|        | $n_{dc}=2$  | 3           | 4           | description                                                       |
|--------|-------------|-------------|-------------|-------------------------------------------------------------------|
| CG1N1  | 1.30        | 1.13        | 1.16        | Carbon in cyano group                                             |
| CG1T1  | 1.45        | 1.12        | 1.16        | Alkyne carbon (R-C)                                               |
| CG1T2  | 0.80        | 0.70        | 0.63        | Alkyne carbon (H-C)                                               |
| CG2R71 | 2.32        | 2.41        | 2.00        | 7-membered aromatic carbon (e.g., azulene)                        |
| FGA3   | <b>0.19</b> | <b>0.17</b> | <b>0.15</b> | Aliphatic fluorine, trifluoro group                               |
| FGR1   | <b>0.40</b> | <b>0.29</b> | <b>0.31</b> | Aromatic fluorine                                                 |
| HGA1   | <b>0.34</b> | <b>0.28</b> | <b>0.29</b> | Aliphatic proton, CH                                              |
| HGA2   | <b>0.27</b> | <b>0.21</b> | <b>0.24</b> | Aliphatic proton, CH2                                             |
| HGA3   | <b>0.23</b> | <b>0.20</b> | <b>0.21</b> | Aliphatic proton, CH3                                             |
| HGP1   | <b>0.36</b> | <b>0.31</b> | <b>0.33</b> | Polar hydrogen                                                    |
| HGP4   | <b>0.31</b> | <b>0.22</b> | <b>0.22</b> | Polar hydrogen, neutral conjugated -NH2 group                     |
| HGPAM1 | <b>0.44</b> | <b>0.38</b> | <b>0.37</b> | Polar hydrogen, neutral dimethylamine group                       |
| HGPAM2 | <b>0.27</b> | <b>0.25</b> | <b>0.24</b> | Polar hydrogen, neutral methylamine group                         |
| HGR51  | <b>0.38</b> | <b>0.34</b> | <b>0.39</b> | Nonpolar hydrogen, neutral 5-membered planar ring carbon          |
| HGR52  | <b>0.36</b> | <b>0.32</b> | <b>0.34</b> | Aldehyde hydrogen, formamide hydrogen (RCOH);                     |
| HGR61  | <b>0.41</b> | <b>0.32</b> | <b>0.34</b> | Aromatic hydrogen                                                 |
| HGR62  | <b>0.40</b> | <b>0.31</b> | <b>0.33</b> | Nonpolar hydrogen, neutral 6-membered planar ring                 |
| NG1T1  | <b>0.32</b> | <b>0.27</b> | <b>0.29</b> | Nitrogen in cyano group                                           |
| NG2D1  | 0.88        | 0.76        | 0.78        | Nitrogen in neutral imine                                         |
| NG2R50 | <b>0.48</b> | <b>0.42</b> | <b>0.46</b> | Double-bonded nitrogen in neutral 5-membered planar ring          |
| NG2R60 | 0.57        | <b>0.47</b> | <b>0.49</b> | Double-bonded nitrogen in neutral 6-membered planar ring          |
| NG2R62 | 0.61        | <b>0.48</b> | <b>0.49</b> | Double-bonded nitrogen in 6-membered planar ring with heteroatoms |
| NG321  | 1.28        | 1.21        | 1.18        | Neutral methylamine nitrogen                                      |
| OG2D1  | <b>0.45</b> | <b>0.37</b> | <b>0.39</b> | Carbonyl oxygen                                                   |
| OG2D4  | <b>0.47</b> | <b>0.37</b> | <b>0.37</b> | 6-membered aromatic carbonyl oxygen                               |
| OG2R50 | 0.58        | 0.50        | 0.57        | Oxygen in furan ring                                              |
| OG301  | 0.99        | 0.80        | 0.79        | Ether oxygen                                                      |
| OG311  | 0.56        | <b>0.45</b> | <b>0.48</b> | Hydroxyl oxygen                                                   |
| OG3R60 | 0.76        | 0.62        | 0.63        | Oxygen in 6-membered cyclic enol, ether, or ester                 |

## S4 Notes on Least Squares Fitting to the ESP

There are a couple of pitfalls when working with ESP data. Firstly, the topology of the grid and the way in which the points are selected can introduce systematic shifts in the magnitude of the charges as well as the ESP, similar to long-range calculations of electrostatics when working with Cartesian-based grids versus radial and angular grids. Other qualitative changes in the orientation/magnitude of the charges can be observed. Secondly, the ESP is not a linear function of the charges, so the RMSE is not a linear function of the charges. This means that the RMSE is not a good measure of the quality of the model. Ultimately, the best test will depend on the application. If these charges are intended from a molecular dynamics simulations of molecules in the condensed phase, as seen in the literature surrounding models like TIP4 and TIP5, the orientation of the charges can have an impact on structural features such as the radial distribution function but perhaps more importantly these choices can have an impact on the future performance of the model when optimizing for other properties. In general, radial/angular grids seem to be preferable to Cartesian grids, especially when using distributed charges when attempting to reproduce the molecular dipole moment; however, it is likely both have strengths and weaknesses and a combination of both may be preferable.

## References

- (1) Bronstein, M. M.; Bruna, J.; LeCun, Y.; Szlam, A.; Vandergheynst, P. Geometric deep learning: going beyond Euclidean data. *IEEE Signal Process. Mag.* **2017**, *34*, 1842, arXiv:1611.08097 [cs].
- (2) Schütt, K.; Unke, O.; Gastegger, M. Equivariant message passing for the prediction of tensorial properties and molecular spectra. Proceedings of the 38th International Conference on Machine Learning. 2021; p 93779388.
- (3) Batatia, I.; Batzner, S.; Kovács, D. P.; Musaelian, A.; Simm, G. N. C.; Drautz, R.; Ort-

- ner, C.; Kozinsky, B.; Csányi, G. The Design Space of E(3)-Equivariant Atom-Centered Interatomic Potentials. **2022**, arXiv:2205.06643 [cond-mat, physics:physics, stat].
- (4) Pozdnyakov, S. N.; Ceriotti, M. Smooth, exact rotational symmetrization for deep learning on point clouds. **2023**, arXiv:2305.19302 [cond-mat, physics:physics].
- (5) Zare, R. N. *Angular Momentum: Understanding Spatial Aspects in Chemistry and Physics*; John Wiley & Sons, 1988.
- (6) Itza Vazquez-Salazar, L.; D. Boittier, E.; Meuwly, M. Uncertainty quantification for predictions of atomistic neural networks. *Chem. Sci.* **2022**, *13*, 1306813084.
- (7) Amari, S.-i. A universal theorem on learning curves. *Neural Networks* **1993**, *6*, 161166.
- (8) Faber, F. A.; Christensen, A. S.; Huang, B.; von Lilienfeld, O. A. Alchemical and structural distribution based representation for universal quantum machine learning. *J. Chem. Phys.* **2018**, *148*, 241717.
